# Supplementary material for: Classical bridge functions in classical and quantum plasma liquids
Source: arXiv:2107.03537 ancillary file (2022-05-17)
Supplement: Supplementary file 1 [file supplementary_material_final.pdf]

# Classical bridge functions in classical and quantum plasma liquids
# Supplemental material

F. Lucco Castello[1], P. Tolias[1] and T. Dornheim[2,3]
[1] *Space and Plasma Physics - Royal Institute of Technology (KTH), SE-10044 Stockholm, Sweden*
[2] *Center for Advanced Systems Understanding (CASUS), D-02826 Görlitz, Germany*
[3] *Helmholtz-Zentrum Dresden-Rossendorf (HZDR), D-01328 Dresden, Germany*

Supplemental material for the manuscript entitled "Classical bridge functions in classical and quantum plasma liquids". Radial distribution functions and bridge functions of Yukawa one-component plasmas as obtained from computer simulations and three integral equation theory approaches: the updated version of the isomorph-based empirically modified hypernetted chain approach, the variational modified hypernetted-chain approach & the empirically modified hypernetted-chain approach. Interaction energies of the unpolarized electron liquid as obtained from computer simulations and three theoretical approaches: the classical mapping method, the hypernetted-chain approach based dielectric scheme and the integral equation theory based dielectric scheme.

## Contents

**Tables 1a-1c**: Key figures of merit of the YOCP radial distribution function, results for $arg_r\{g(r) = 0.5\}$. Each table provides the results for a value of the screening parameter belonging to the set $\kappa = \{0, 1, 2\}$.

**Tables 2a-2c**: Key figures of merit of the YOCP radial distribution function, results for *the magnitude of the first maximum*. Each table provides the results for a value of the screening parameter belonging to the set $\kappa = \{0, 1, 2\}$.

**Tables 3a-3c**: Key figures of merit of the YOCP radial distribution function, results for *the position of the first maximum*. Each table provides the results for a value of the screening parameter belonging to the set $\kappa = \{0, 1, 2\}$.

**Tables 4a-4c**: Key figures of merit of the YOCP radial distribution function, results for *the magnitude of the first non-zero minimum*. Each table provides the results for a value of the screening parameter belonging to the set $\kappa = \{0, 1, 2\}$.

**Tables 5a-5c**: Key figures of merit of the YOCP radial distribution function, results for *the position of the first non-zero minimum*. Each table provides the results for a value of the screening parameter belonging to the set $\kappa = \{0, 1, 2\}$.

**Tables 6a-6c**: Key figures of merit of the YOCP radial distribution function, results for *the magnitude of the second maximum*. Each table provides the results for a value of the screening parameter belonging to the set $\kappa = \{0, 1, 2\}$.

**Tables 7a-7c**: Key figures of merit of the YOCP radial distribution function, results for *the position of the second maximum*. Each table provides the results for a value of the screening parameter belonging to the set $\kappa = \{0, 1, 2\}$.

**Figure 1**: YOCP bridge functions in the entire non-trivial range. Results for four isomorphic state points with a reduced excess entropy $s_{\mathrm{ex}} = -3.880$.

**Figure 2**: YOCP bridge functions in the entire non-trivial range. Results for four isomorphic state points with a reduced excess entropy $s_{\mathrm{ex}} = -3.380$.

**Figure 3**: YOCP bridge functions in the entire non-trivial range. Results for four isomorphic state points with a reduced excess entropy $s_{\mathrm{ex}} = -2.764$.

**Figure 4**: YOCP bridge functions in the entire non-trivial range. Results for four isomorphic state points with a reduced excess entropy $s_{\mathrm{ex}} = -1.918$.

**Table 8**: Interaction energies of the unpolarized electron liquid. Results for twenty thermodynamic states.

**Table 1a.** Key properties of the radial distribution function as resulting from molecular dynamics (MD) simulations and from three integral equation theory approaches: the updated version of the isomorph-based empirically modified hypernetted chain approximation (IEMHNC) introduced in the present letter, the variational modified hypernetted-chain approximation (VMHNC) discussed in *G. Faussurier, Phys. Rev. E* **69**, *066402 (2004)* and the empirically modified hypernetted-chain approximation (EMHNC) presented in *W. Daughton, M. S. Murillo and L. Thode, Phys. Rev. E* **61**, *2129 (2000)*. The absolute relative deviation $\epsilon_{\mathrm{r}}$ between the theoretical and the simulation results is also reported together with its average and maximum values (the average deviation is denoted as $\epsilon_{\mathrm{AVE}}$ and the maximum deviation is denoted as $\epsilon_{\mathrm{MAX}}$). **Results for $\arg_r\{g(r)=0.5\}$ in the case of $\kappa=0.0$**. The MD results are adopted from *T. Ott and M. Bonitz, Contrib. Plasma Phys.* **55**, *243 (2015)*. Here $x=r/d$, where $d$ is the Wigner-Seitz radius.

| $\Gamma$ | $\Gamma/\Gamma_m$ | $x_{\mathrm{cv}}^{\mathrm{MD}}$ | $x_{\mathrm{cv}}^{\mathrm{IEMHNC}}$ | $\epsilon_{\mathrm{IEMHNC}}(\%)$ | $x_{\mathrm{cv}}^{\mathrm{VMHNC}}$ | $\epsilon_{\mathrm{VMHNC}}(\%)$ | $x_{\mathrm{cv}}^{\mathrm{EMHNC}}$ | $\epsilon_{\mathrm{EMHNC}}(\%)$ |
|---|---|---|---|---|---|---|---|---|
| 15.0 | 0.09 | 1.179 | 1.178 | 0.085 | 1.176 | 0.254 | 1.165 | 1.187 |
| 20.0 | 0.12 | 1.218 | 1.217 | 0.082 | 1.217 | 0.082 | 1.207 | 0.903 |
| 25.0 | 0.15 | 1.246 | 1.245 | 0.080 | 1.247 | 0.080 | 1.237 | 0.722 |
| 30.0 | 0.17 | 1.272 | 1.268 | 0.314 | 1.271 | 0.079 | 1.262 | 0.786 |
| 35.0 | 0.20 | 1.291 | 1.288 | 0.232 | 1.291 | 0.000 | 1.282 | 0.697 |
| 40.0 | 0.23 | 1.307 | 1.304 | 0.230 | 1.307 | 0.000 | 1.299 | 0.612 |
| 45.0 | 0.26 | 1.320 | 1.319 | 0.076 | 1.322 | 0.152 | 1.314 | 0.455 |
| 50.0 | 0.29 | 1.333 | 1.332 | 0.075 | 1.335 | 0.150 | 1.327 | 0.450 |
| 55.0 | 0.32 | 1.346 | 1.343 | 0.223 | 1.346 | 0.000 | 1.338 | 0.594 |
| 60.0 | 0.35 | 1.355 | 1.354 | 0.074 | 1.356 | 0.074 | 1.349 | 0.443 |
| 65.0 | 0.38 | 1.365 | 1.363 | 0.147 | 1.366 | 0.073 | 1.359 | 0.440 |
| 70.0 | 0.41 | 1.374 | 1.372 | 0.146 | 1.374 | 0.000 | 1.367 | 0.509 |
| 75.0 | 0.44 | 1.381 | 1.380 | 0.072 | 1.382 | 0.072 | 1.376 | 0.362 |
| 80.0 | 0.47 | 1.387 | 1.387 | 0.000 | 1.390 | 0.216 | 1.383 | 0.288 |
| 85.0 | 0.49 | 1.394 | 1.394 | 0.000 | 1.396 | 0.143 | 1.390 | 0.287 |
| 90.0 | 0.52 | 1.400 | 1.401 | 0.071 | 1.403 | 0.214 | 1.397 | 0.214 |
| 95.0 | 0.55 | 1.406 | 1.407 | 0.071 | 1.409 | 0.213 | 1.403 | 0.213 |
| 100.0 | 0.58 | 1.413 | 1.412 | 0.071 | 1.414 | 0.071 | 1.409 | 0.283 |
| 105.0 | 0.61 | 1.419 | 1.418 | 0.070 | 1.420 | 0.070 | 1.415 | 0.282 |
| 110.0 | 0.64 | 1.422 | 1.423 | 0.070 | 1.425 | 0.211 | 1.420 | 0.141 |
| 115.0 | 0.67 | 1.429 | 1.428 | 0.070 | 1.429 | 0.000 | 1.425 | 0.280 |
| 120.0 | 0.70 | 1.432 | 1.432 | 0.000 | 1.434 | 0.140 | 1.430 | 0.140 |
| 125.0 | 0.73 | 1.435 | 1.437 | 0.139 | 1.438 | 0.209 | 1.434 | 0.070 |
| 130.0 | 0.76 | 1.442 | 1.441 | 0.069 | 1.442 | 0.000 | 1.439 | 0.208 |
| 135.0 | 0.79 | 1.445 | 1.445 | 0.000 | 1.446 | 0.069 | 1.443 | 0.138 |
| 140.0 | 0.81 | 1.448 | 1.449 | 0.069 | 1.450 | 0.138 | 1.447 | 0.069 |
| 145.0 | 0.84 | 1.451 | 1.452 | 0.069 | 1.454 | 0.207 | 1.451 | 0.000 |
| 150.0 | 0.87 | 1.454 | 1.456 | 0.138 | 1.457 | 0.206 | 1.455 | 0.069 |
| 155.0 | 0.90 | 1.461 | 1.459 | 0.137 | 1.461 | 0.000 | 1.458 | 0.205 |
| 160.0 | 0.93 | 1.464 | 1.462 | 0.137 | 1.464 | 0.000 | 1.462 | 0.137 |
| $\epsilon_{\mathrm{AVE}}(\%)$ | | | | **0.101** | | **0.104** | | **0.373** |
| $\epsilon_{\mathrm{MAX}}(\%)$ | | | | **0.314** | | **0.254** | | **1.187** |

**Table 1b.** Key properties of the radial distribution function as resulting from molecular dynamics (MD) simulations and from three integral equation theory approaches: the updated version of the isomorph-based empirically modified hypernetted chain approximation (IEMHNC) introduced in the present letter, the variational modified hypernetted-chain approximation (VMHNC) discussed in *G. Faussurier, Phys. Rev. E* **69**, *066402 (2004)* and the empirically modified hypernetted-chain approximation (EMHNC) presented in *W. Daughton, M. S. Murillo and L. Thode, Phys. Rev. E* **61**, *2129 (2000)*. The absolute relative deviation $\epsilon_{\mathrm{r}}$ between the theoretical and the simulation results is also reported together with its average and maximum values (the average deviation is denoted as $\epsilon_{\mathrm{AVE}}$ and the maximum deviation is denoted as $\epsilon_{\mathrm{MAX}}$). **Results for $\arg_r\{g(r)=0.5\}$ in the case of $\kappa=1.0$**. The MD results are adopted from *T. Ott and M. Bonitz, Contrib. Plasma Phys.* **55**, *243 (2015)*. Here $x=r/d$, where $d$ is the Wigner-Seitz radius.

| $\Gamma$ | $\Gamma/\Gamma_m$ | $x_{\mathrm{cv}}^{\mathrm{MD}}$ | $x_{\mathrm{cv}}^{\mathrm{IEMHNC}}$ | $\epsilon_{\mathrm{IEMHNC}}(\%)$ | $x_{\mathrm{cv}}^{\mathrm{VMHNC}}$ | $\epsilon_{\mathrm{VMHNC}}(\%)$ | $x_{\mathrm{cv}}^{\mathrm{EMHNC}}$ | $\epsilon_{\mathrm{EMHNC}}(\%)$ |
|---|---|---|---|---|---|---|---|---|
| 10.0 | 0.05 | 1.076 | 1.071 | 0.465 | 1.070 | 0.558 | 1.062 | 1.301 |
| 15.0 | 0.07 | 1.139 | 1.137 | 0.176 | 1.134 | 0.439 | 1.128 | 0.966 |
| 20.0 | 0.09 | 1.177 | 1.180 | 0.255 | 1.177 | 0.000 | 1.172 | 0.425 |
| 25.0 | 0.11 | 1.211 | 1.211 | 0.000 | 1.209 | 0.165 | 1.204 | 0.578 |
| 30.0 | 0.14 | 1.237 | 1.235 | 0.162 | 1.234 | 0.243 | 1.230 | 0.566 |
| 35.0 | 0.16 | 1.254 | 1.255 | 0.080 | 1.255 | 0.080 | 1.251 | 0.239 |
| 40.0 | 0.18 | 1.275 | 1.272 | 0.235 | 1.273 | 0.157 | 1.269 | 0.471 |
| 45.0 | 0.20 | 1.288 | 1.287 | 0.078 | 1.288 | 0.000 | 1.284 | 0.311 |
| 50.0 | 0.23 | 1.301 | 1.300 | 0.077 | 1.302 | 0.077 | 1.298 | 0.231 |
| 55.0 | 0.25 | 1.313 | 1.312 | 0.076 | 1.314 | 0.076 | 1.310 | 0.228 |
| 60.0 | 0.27 | 1.326 | 1.323 | 0.226 | 1.325 | 0.075 | 1.321 | 0.377 |
| 65.0 | 0.30 | 1.334 | 1.333 | 0.075 | 1.335 | 0.075 | 1.331 | 0.225 |
| 70.0 | 0.32 | 1.343 | 1.342 | 0.074 | 1.344 | 0.074 | 1.340 | 0.223 |
| 75.0 | 0.34 | 1.351 | 1.351 | 0.000 | 1.352 | 0.074 | 1.348 | 0.222 |
| 80.0 | 0.36 | 1.360 | 1.358 | 0.147 | 1.360 | 0.000 | 1.356 | 0.294 |
| 85.0 | 0.39 | 1.364 | 1.366 | 0.147 | 1.367 | 0.220 | 1.364 | 0.000 |
| 90.0 | 0.41 | 1.373 | 1.372 | 0.073 | 1.373 | 0.000 | 1.370 | 0.218 |
| 95.0 | 0.43 | 1.377 | 1.379 | 0.145 | 1.380 | 0.218 | 1.377 | 0.000 |
| 100.0 | 0.45 | 1.385 | 1.385 | 0.000 | 1.386 | 0.072 | 1.383 | 0.144 |
| 105.0 | 0.48 | 1.390 | 1.390 | 0.000 | 1.391 | 0.072 | 1.389 | 0.072 |
| 110.0 | 0.50 | 1.394 | 1.396 | 0.143 | 1.397 | 0.215 | 1.394 | 0.000 |
| 115.0 | 0.52 | 1.402 | 1.401 | 0.071 | 1.402 | 0.000 | 1.399 | 0.214 |
| 120.0 | 0.54 | 1.407 | 1.406 | 0.071 | 1.406 | 0.071 | 1.404 | 0.213 |
| 125.0 | 0.57 | 1.411 | 1.410 | 0.071 | 1.411 | 0.000 | 1.409 | 0.142 |
| 130.0 | 0.59 | 1.415 | 1.414 | 0.071 | 1.415 | 0.000 | 1.414 | 0.071 |
| 135.0 | 0.61 | 1.419 | 1.419 | 0.000 | 1.419 | 0.000 | 1.418 | 0.070 |
| 140.0 | 0.64 | 1.424 | 1.423 | 0.070 | 1.423 | 0.070 | 1.422 | 0.140 |
| 145.0 | 0.66 | 1.428 | 1.427 | 0.070 | 1.427 | 0.070 | 1.426 | 0.140 |
| 150.0 | 0.68 | 1.428 | 1.430 | 0.140 | 1.431 | 0.210 | 1.430 | 0.140 |
| 155.0 | 0.70 | 1.432 | 1.434 | 0.140 | 1.434 | 0.140 | 1.434 | 0.140 |
| 160.0 | 0.73 | 1.436 | 1.437 | 0.070 | 1.438 | 0.139 | 1.438 | 0.139 |
| 165.0 | 0.75 | 1.441 | 1.440 | 0.069 | 1.441 | 0.000 | 1.441 | 0.000 |
| 170.0 | 0.77 | 1.445 | 1.444 | 0.069 | 1.444 | 0.069 | 1.444 | 0.069 |
| 175.0 | 0.79 | 1.445 | 1.447 | 0.138 | 1.447 | 0.138 | 1.448 | 0.208 |
| 180.0 | 0.82 | 1.449 | 1.450 | 0.069 | 1.450 | 0.069 | 1.451 | 0.138 |
| 185.0 | 0.84 | 1.453 | 1.453 | 0.000 | 1.453 | 0.000 | 1.454 | 0.069 |
| 190.0 | 0.86 | 1.453 | 1.455 | 0.138 | 1.456 | 0.206 | 1.457 | 0.275 |
| 195.0 | 0.89 | 1.458 | 1.458 | 0.000 | 1.459 | 0.069 | 1.460 | 0.137 |
| 200.0 | 0.91 | 1.462 | 1.461 | 0.068 | 1.461 | 0.068 | 1.463 | 0.068 |
| $\boldsymbol{\epsilon_{\mathrm{AVE}}}(\%)$ | | | | **0.102** | | **0.108** | | **0.243** |
| $\boldsymbol{\epsilon_{\mathrm{MAX}}}(\%)$ | | | | **0.465** | | **0.558** | | **1.301** |

**Table 1c.** Key properties of the radial distribution function as resulting from molecular dynamics (MD) simulations and from three integral equation theory approaches: the updated version of the isomorph-based empirically modified hypernetted chain approximation (IEMHNC) introduced in the present letter, the variational modified hypernetted-chain approximation (VMHNC) discussed in *G. Faussurier, Phys. Rev. E* **69**, *066402 (2004)* and the empirically modified hypernetted-chain approximation (EMHNC) presented in *W. Daughton, M. S. Murillo and L. Thode, Phys. Rev. E* **61**, *2129 (2000)*. The absolute relative deviation $\epsilon_{\mathrm{r}}$ between the theoretical and the simulation results is also reported together with its average and maximum values (the average deviation is denoted as $\epsilon_{\mathrm{AVE}}$ and the maximum deviation is denoted as $\epsilon_{\mathrm{MAX}}$). **Results for $\arg_r\{g(r)=0.5\}$ in the case of $\kappa=2.0$**. The MD results are adopted from *T. Ott and M. Bonitz, Contrib. Plasma Phys.* **55**, *243 (2015)*. Here $x=r/d$, where $d$ is the Wigner-Seitz radius.

| $\Gamma$ | $\Gamma/\Gamma_m$ | $x_{\mathrm{cv}}^{\mathrm{MD}}$ | $x_{\mathrm{cv}}^{\mathrm{IEMHNC}}$ | $\epsilon_{\mathrm{IEMHNC}}(\%)$ | $x_{\mathrm{cv}}^{\mathrm{VMHNC}}$ | $\epsilon_{\mathrm{VMHNC}}(\%)$ | $x_{\mathrm{cv}}^{\mathrm{EMHNC}}$ | $\epsilon_{\mathrm{EMHNC}}(\%)$ |
|---|---|---|---|---|---|---|---|---|
| 30.0 | 0.07 | 1.135 | 1.135 | 0.000 | 1.133 | 0.176 | 1.136 | 0.088 |
| 40.0 | 0.09 | 1.176 | 1.178 | 0.170 | 1.176 | 0.000 | 1.179 | 0.255 |
| 50.0 | 0.11 | 1.209 | 1.209 | 0.000 | 1.208 | 0.083 | 1.211 | 0.165 |
| 60.0 | 0.13 | 1.234 | 1.234 | 0.000 | 1.234 | 0.000 | 1.236 | 0.162 |
| 70.0 | 0.15 | 1.254 | 1.254 | 0.000 | 1.255 | 0.080 | 1.257 | 0.239 |
| 80.0 | 0.17 | 1.272 | 1.272 | 0.000 | 1.273 | 0.079 | 1.275 | 0.236 |
| 90.0 | 0.20 | 1.288 | 1.287 | 0.078 | 1.288 | 0.000 | 1.291 | 0.233 |
| 100.0 | 0.22 | 1.301 | 1.300 | 0.077 | 1.302 | 0.077 | 1.304 | 0.231 |
| 110.0 | 0.24 | 1.313 | 1.312 | 0.076 | 1.314 | 0.076 | 1.317 | 0.305 |
| 120.0 | 0.26 | 1.324 | 1.323 | 0.076 | 1.325 | 0.076 | 1.328 | 0.302 |
| 130.0 | 0.28 | 1.333 | 1.334 | 0.075 | 1.335 | 0.150 | 1.338 | 0.375 |
| 140.0 | 0.31 | 1.342 | 1.343 | 0.075 | 1.344 | 0.149 | 1.347 | 0.373 |
| 150.0 | 0.33 | 1.351 | 1.351 | 0.000 | 1.353 | 0.148 | 1.356 | 0.370 |
| 160.0 | 0.35 | 1.358 | 1.359 | 0.074 | 1.360 | 0.147 | 1.363 | 0.368 |
| 170.0 | 0.37 | 1.366 | 1.366 | 0.000 | 1.368 | 0.146 | 1.371 | 0.366 |
| 180.0 | 0.39 | 1.373 | 1.373 | 0.000 | 1.375 | 0.146 | 1.378 | 0.364 |
| 190.0 | 0.41 | 1.378 | 1.380 | 0.145 | 1.381 | 0.218 | 1.384 | 0.435 |
| 200.0 | 0.44 | 1.384 | 1.386 | 0.145 | 1.387 | 0.217 | 1.391 | 0.506 |
| 210.0 | 0.46 | 1.389 | 1.391 | 0.144 | 1.393 | 0.288 | 1.397 | 0.576 |
| 220.0 | 0.48 | 1.396 | 1.397 | 0.072 | 1.398 | 0.143 | 1.402 | 0.430 |
| 230.0 | 0.50 | 1.400 | 1.402 | 0.143 | 1.403 | 0.214 | 1.407 | 0.500 |
| 240.0 | 0.52 | 1.405 | 1.407 | 0.142 | 1.408 | 0.214 | 1.412 | 0.498 |
| 250.0 | 0.55 | 1.409 | 1.411 | 0.142 | 1.413 | 0.284 | 1.417 | 0.568 |
| 260.0 | 0.57 | 1.414 | 1.416 | 0.141 | 1.417 | 0.212 | 1.422 | 0.566 |
| 270.0 | 0.59 | 1.418 | 1.420 | 0.141 | 1.421 | 0.212 | 1.426 | 0.564 |
| 280.0 | 0.61 | 1.423 | 1.424 | 0.070 | 1.425 | 0.141 | 1.431 | 0.562 |
| 290.0 | 0.63 | 1.427 | 1.428 | 0.070 | 1.429 | 0.140 | 1.435 | 0.561 |
| 300.0 | 0.65 | 1.429 | 1.432 | 0.210 | 1.433 | 0.280 | 1.439 | 0.700 |
| 310.0 | 0.68 | 1.434 | 1.435 | 0.070 | 1.436 | 0.139 | 1.442 | 0.558 |
| 320.0 | 0.70 | 1.436 | 1.439 | 0.209 | 1.440 | 0.279 | 1.446 | 0.696 |
| 330.0 | 0.72 | 1.441 | 1.442 | 0.069 | 1.443 | 0.139 | 1.449 | 0.555 |
| 340.0 | 0.74 | 1.443 | 1.445 | 0.139 | 1.446 | 0.208 | 1.453 | 0.693 |
| 350.0 | 0.76 | 1.447 | 1.448 | 0.069 | 1.450 | 0.207 | 1.456 | 0.622 |
| 360.0 | 0.79 | 1.450 | 1.451 | 0.069 | 1.453 | 0.207 | 1.459 | 0.621 |
| 370.0 | 0.81 | 1.452 | 1.454 | 0.138 | 1.456 | 0.275 | 1.462 | 0.689 |
| 380.0 | 0.83 | 1.456 | 1.457 | 0.069 | 1.458 | 0.137 | 1.465 | 0.618 |
| 390.0 | 0.85 | 1.459 | 1.460 | 0.069 | 1.461 | 0.137 | 1.468 | 0.617 |
| 400.0 | 0.87 | 1.461 | 1.462 | 0.068 | 1.464 | 0.205 | 1.471 | 0.684 |
| $\boldsymbol{\epsilon_{\mathrm{AVE}}}(\%)$ | | | | **0.085** | | **0.159** | | **0.454** |
| $\boldsymbol{\epsilon_{\mathrm{MAX}}}(\%)$ | | | | **0.210** | | **0.288** | | **0.700** |

**Table 2a.** Key properties of the radial distribution function as resulting from molecular dynamics (MD) simulations and from three integral equation theory approaches: the updated version of the isomorph-based empirically modified hypernetted chain approximation (IEMHNC) introduced in the present letter, the variational modified hypernetted-chain approximation (VMHNC) discussed in *G. Faussurier, Phys. Rev. E* **69**, *066402 (2004)* and the empirically modified hypernetted-chain approximation (EMHNC) presented in *W. Daughton, M. S. Murillo and L. Thode, Phys. Rev. E* **61**, *2129 (2000)*. The absolute relative deviation $\epsilon_{\mathrm{r}}$ between the theoretical and the simulation results is also reported together with its average and maximum values (the average deviation is denoted as $\epsilon_{\mathrm{AVE}}$ and the maximum deviation is denoted as $\epsilon_{\mathrm{MAX}}$). **Results for the magnitude of the first maximum in the case of $\boldsymbol{\kappa = 0.0}$**. The MD results are adopted from *T. Ott and M. Bonitz, Contrib. Plasma Phys.* **55**, *243 (2015)*.

| $\Gamma$ | $\Gamma/\Gamma_m$ | $g_{\mathrm{max1}}^{\mathrm{MD}}$ | $g_{\mathrm{max1}}^{\mathrm{IEMHNC}}$ | $\epsilon_{\mathrm{IEMHNC}}(\%)$ | $g_{\mathrm{max1}}^{\mathrm{VMHNC}}$ | $\epsilon_{\mathrm{VMHNC}}(\%)$ | $g_{\mathrm{max1}}^{\mathrm{EMHNC}}$ | $\epsilon_{\mathrm{EMHNC}}(\%)$ |
|---|---|---|---|---|---|---|---|---|
| 15.0 | 0.09 | 1.228 | 1.227 | 0.081 | 1.228 | 0.000 | 1.200 | 2.280 |
| 20.0 | 0.12 | 1.307 | 1.307 | 0.000 | 1.312 | 0.383 | 1.277 | 2.295 |
| 25.0 | 0.15 | 1.378 | 1.378 | 0.000 | 1.387 | 0.653 | 1.348 | 2.177 |
| 30.0 | 0.17 | 1.443 | 1.442 | 0.069 | 1.457 | 0.970 | 1.414 | 2.010 |
| 35.0 | 0.20 | 1.504 | 1.502 | 0.133 | 1.521 | 1.130 | 1.475 | 1.928 |
| 40.0 | 0.23 | 1.560 | 1.557 | 0.192 | 1.581 | 1.346 | 1.533 | 1.731 |
| 45.0 | 0.26 | 1.614 | 1.610 | 0.248 | 1.637 | 1.425 | 1.587 | 1.673 |
| 50.0 | 0.29 | 1.664 | 1.661 | 0.180 | 1.691 | 1.623 | 1.639 | 1.502 |
| 55.0 | 0.32 | 1.712 | 1.709 | 0.175 | 1.741 | 1.694 | 1.688 | 1.402 |
| 60.0 | 0.35 | 1.757 | 1.755 | 0.114 | 1.790 | 1.878 | 1.735 | 1.252 |
| 65.0 | 0.38 | 1.803 | 1.799 | 0.222 | 1.837 | 1.886 | 1.781 | 1.220 |
| 70.0 | 0.41 | 1.845 | 1.842 | 0.163 | 1.881 | 1.951 | 1.824 | 1.138 |
| 75.0 | 0.44 | 1.885 | 1.884 | 0.053 | 1.925 | 2.122 | 1.867 | 0.955 |
| 80.0 | 0.47 | 1.926 | 1.924 | 0.104 | 1.966 | 2.077 | 1.908 | 0.935 |
| 85.0 | 0.49 | 1.964 | 1.963 | 0.051 | 2.007 | 2.189 | 1.948 | 0.815 |
| 90.0 | 0.52 | 2.001 | 2.001 | 0.000 | 2.046 | 2.249 | 1.987 | 0.700 |
| 95.0 | 0.55 | 2.037 | 2.037 | 0.000 | 2.084 | 2.307 | 2.025 | 0.589 |
| 100.0 | 0.58 | 2.072 | 2.073 | 0.048 | 2.122 | 2.413 | 2.063 | 0.434 |
| 105.0 | 0.61 | 2.107 | 2.108 | 0.047 | 2.158 | 2.421 | 2.099 | 0.380 |
| 110.0 | 0.64 | 2.140 | 2.143 | 0.140 | 2.193 | 2.477 | 2.134 | 0.280 |
| 115.0 | 0.67 | 2.174 | 2.176 | 0.092 | 2.228 | 2.484 | 2.169 | 0.230 |
| 120.0 | 0.70 | 2.206 | 2.209 | 0.136 | 2.262 | 2.539 | 2.204 | 0.091 |
| 125.0 | 0.73 | 2.237 | 2.240 | 0.134 | 2.295 | 2.593 | 2.237 | 0.000 |
| 130.0 | 0.76 | 2.270 | 2.271 | 0.044 | 2.327 | 2.511 | 2.270 | 0.000 |
| 135.0 | 0.79 | 2.298 | 2.302 | 0.174 | 2.359 | 2.654 | 2.303 | 0.218 |
| 140.0 | 0.81 | 2.329 | 2.331 | 0.086 | 2.390 | 2.619 | 2.334 | 0.215 |
| 145.0 | 0.84 | 2.358 | 2.360 | 0.085 | 2.421 | 2.672 | 2.366 | 0.339 |
| 150.0 | 0.87 | 2.386 | 2.388 | 0.084 | 2.451 | 2.724 | 2.397 | 0.461 |
| 155.0 | 0.90 | 2.413 | 2.416 | 0.124 | 2.481 | 2.818 | 2.427 | 0.580 |
| 160.0 | 0.93 | 2.442 | 2.442 | 0.000 | 2.510 | 2.785 | 2.457 | 0.614 |
| $\boldsymbol{\epsilon_{\mathrm{AVE}}}(\%)$ | | | | **0.099** | | **1.986** | | **0.948** |
| $\boldsymbol{\epsilon_{\mathrm{MAX}}}(\%)$ | | | | **0.248** | | **2.818** | | **2.295** |

**Table 2b.** Key properties of the radial distribution function as resulting from molecular dynamics (MD) simulations and from three integral equation theory approaches: the updated version of the isomorph-based empirically modified hypernetted chain approximation (IEMHNC) introduced in the present letter, the variational modified hypernetted-chain approximation (VMHNC) discussed in *G. Faussurier, Phys. Rev. E* **69**, *066402 (2004)* and the empirically modified hypernetted-chain approximation (EMHNC) presented in *W. Daughton, M. S. Murillo and L. Thode, Phys. Rev. E* **61**, *2129 (2000).* The absolute relative deviation $\epsilon_{\mathrm{r}}$ between the theoretical and the simulation results is also reported together with its average and maximum values (the average deviation is denoted as $\epsilon_{\mathrm{AVE}}$ and the maximum deviation is denoted as $\epsilon_{\mathrm{MAX}}$). **Results for the magnitude of the first maximum in the case of $\boldsymbol{\kappa = 1.0}$**. The MD results are adopted from *T. Ott and M. Bonitz, Contrib. Plasma Phys.* **55**, *243 (2015).*

| $\Gamma$ | $\Gamma/\Gamma_m$ | $g_{\mathrm{max1}}^{\mathrm{MD}}$ | $g_{\mathrm{max1}}^{\mathrm{IEMHNC}}$ | $\epsilon_{\mathrm{IEMHNC}}(\%)$ | $g_{\mathrm{max1}}^{\mathrm{VMHNC}}$ | $\epsilon_{\mathrm{VMHNC}}(\%)$ | $g_{\mathrm{max1}}^{\mathrm{EMHNC}}$ | $\epsilon_{\mathrm{EMHNC}}(\%)$ |
|---|---|---|---|---|---|---|---|---|
| 10.0 | 0.05 | 1.101 | 1.100 | 0.091 | 1.097 | 0.363 | 1.089 | 1.090 |
| 15.0 | 0.07 | 1.175 | 1.176 | 0.085 | 1.174 | 0.085 | 1.159 | 1.362 |
| 20.0 | 0.09 | 1.243 | 1.246 | 0.241 | 1.245 | 0.161 | 1.225 | 1.448 |
| 25.0 | 0.11 | 1.304 | 1.309 | 0.383 | 1.310 | 0.460 | 1.288 | 1.227 |
| 30.0 | 0.14 | 1.360 | 1.365 | 0.368 | 1.370 | 0.735 | 1.345 | 1.103 |
| 35.0 | 0.16 | 1.413 | 1.418 | 0.354 | 1.426 | 0.920 | 1.400 | 0.920 |
| 40.0 | 0.18 | 1.462 | 1.466 | 0.274 | 1.478 | 1.094 | 1.450 | 0.821 |
| 45.0 | 0.20 | 1.509 | 1.513 | 0.265 | 1.528 | 1.259 | 1.499 | 0.663 |
| 50.0 | 0.23 | 1.553 | 1.557 | 0.258 | 1.575 | 1.417 | 1.544 | 0.580 |
| 55.0 | 0.25 | 1.595 | 1.599 | 0.251 | 1.619 | 1.505 | 1.588 | 0.439 |
| 60.0 | 0.27 | 1.636 | 1.640 | 0.244 | 1.662 | 1.589 | 1.630 | 0.367 |
| 65.0 | 0.30 | 1.675 | 1.679 | 0.239 | 1.704 | 1.731 | 1.670 | 0.299 |
| 70.0 | 0.32 | 1.711 | 1.717 | 0.351 | 1.743 | 1.870 | 1.709 | 0.117 |
| 75.0 | 0.34 | 1.749 | 1.753 | 0.229 | 1.781 | 1.830 | 1.747 | 0.114 |
| 80.0 | 0.36 | 1.783 | 1.789 | 0.337 | 1.818 | 1.963 | 1.784 | 0.056 |
| 85.0 | 0.39 | 1.817 | 1.823 | 0.330 | 1.854 | 2.036 | 1.819 | 0.110 |
| 90.0 | 0.41 | 1.850 | 1.857 | 0.378 | 1.889 | 2.108 | 1.854 | 0.216 |
| 95.0 | 0.43 | 1.882 | 1.890 | 0.425 | 1.923 | 2.179 | 1.888 | 0.319 |
| 100.0 | 0.45 | 1.914 | 1.921 | 0.366 | 1.956 | 2.194 | 1.921 | 0.366 |
| 105.0 | 0.48 | 1.944 | 1.953 | 0.463 | 1.988 | 2.263 | 1.953 | 0.463 |
| 110.0 | 0.50 | 1.974 | 1.983 | 0.456 | 2.020 | 2.330 | 1.985 | 0.557 |
| 115.0 | 0.52 | 2.003 | 2.013 | 0.499 | 2.051 | 2.396 | 2.016 | 0.649 |
| 120.0 | 0.54 | 2.031 | 2.042 | 0.542 | 2.081 | 2.462 | 2.046 | 0.739 |
| 125.0 | 0.57 | 2.058 | 2.070 | 0.583 | 2.110 | 2.527 | 2.076 | 0.875 |
| 130.0 | 0.59 | 2.088 | 2.098 | 0.479 | 2.139 | 2.443 | 2.106 | 0.862 |
| 135.0 | 0.61 | 2.114 | 2.126 | 0.568 | 2.167 | 2.507 | 2.134 | 0.946 |
| 140.0 | 0.64 | 2.141 | 2.153 | 0.560 | 2.195 | 2.522 | 2.163 | 1.028 |
| 145.0 | 0.66 | 2.166 | 2.179 | 0.600 | 2.222 | 2.585 | 2.191 | 1.154 |
| 150.0 | 0.68 | 2.191 | 2.205 | 0.639 | 2.249 | 2.647 | 2.218 | 1.232 |
| 155.0 | 0.70 | 2.217 | 2.230 | 0.586 | 2.276 | 2.661 | 2.245 | 1.263 |
| 160.0 | 0.73 | 2.242 | 2.255 | 0.580 | 2.302 | 2.676 | 2.272 | 1.338 |
| 165.0 | 0.75 | 2.266 | 2.280 | 0.618 | 2.327 | 2.692 | 2.299 | 1.456 |
| 170.0 | 0.77 | 2.289 | 2.304 | 0.655 | 2.352 | 2.752 | 2.325 | 1.573 |
| 175.0 | 0.79 | 2.314 | 2.327 | 0.562 | 2.377 | 2.723 | 2.350 | 1.556 |
| 180.0 | 0.82 | 2.337 | 2.350 | 0.556 | 2.402 | 2.781 | 2.376 | 1.669 |
| 185.0 | 0.84 | 2.359 | 2.373 | 0.593 | 2.426 | 2.840 | 2.401 | 1.780 |
| 190.0 | 0.86 | 2.383 | 2.395 | 0.504 | 2.450 | 2.812 | 2.425 | 1.762 |
| 195.0 | 0.89 | 2.404 | 2.417 | 0.541 | 2.473 | 2.870 | 2.450 | 1.913 |
| 200.0 | 0.91 | 2.427 | 2.439 | 0.494 | 2.496 | 2.843 | 2.474 | 1.937 |
| $\boldsymbol{\epsilon_{\mathrm{AVE}}}(\%)$ | | | | **0.424** | | **1.996** | | **0.932** |
| $\boldsymbol{\epsilon_{\mathrm{MAX}}}(\%)$ | | | | **0.655** | | **2.870** | | **1.937** |

**Table 2c.** Key properties of the radial distribution function as resulting from molecular dynamics (MD) simulations and from three integral equation theory approaches: the updated version of the isomorph-based empirically modified hypernetted chain approximation (IEMHNC) introduced in the present letter, the variational modified hypernetted-chain approximation (VMHNC) discussed in *G. Faussurier, Phys. Rev. E* **69**, *066402 (2004)* and the empirically modified hypernetted-chain approximation (EMHNC) presented in *W. Daughton, M. S. Murillo and L. Thode, Phys. Rev. E* **61**, *2129 (2000)*. The absolute relative deviation $\epsilon_{\mathrm{r}}$ between the theoretical and the simulation results is also reported together with its average and maximum values (the average deviation is denoted as $\epsilon_{\mathrm{AVE}}$ and the maximum deviation is denoted as $\epsilon_{\mathrm{MAX}}$). **Results for the magnitude of the first maximum in the case of $\boldsymbol{\kappa = 2.0}$**. The MD results are adopted from *T. Ott and M. Bonitz, Contrib. Plasma Phys.* **55**, *243 (2015)*.

| $\Gamma$ | $\Gamma/\Gamma_m$ | $g_{\mathrm{max1}}^{\mathrm{MD}}$ | $g_{\mathrm{max1}}^{\mathrm{IEMHNC}}$ | $\epsilon_{\mathrm{IEMHNC}}(\%)$ | $g_{\mathrm{max1}}^{\mathrm{VMHNC}}$ | $\epsilon_{\mathrm{VMHNC}}(\%)$ | $g_{\mathrm{max1}}^{\mathrm{EMHNC}}$ | $\epsilon_{\mathrm{EMHNC}}(\%)$ |
|---|---|---|---|---|---|---|---|---|
| 30.0 | 0.07 | 1.202 | 1.202 | 0.000 | 1.206 | 0.333 | 1.201 | 0.083 |
| 40.0 | 0.09 | 1.270 | 1.274 | 0.315 | 1.277 | 0.551 | 1.273 | 0.236 |
| 50.0 | 0.11 | 1.331 | 1.337 | 0.451 | 1.342 | 0.826 | 1.337 | 0.451 |
| 60.0 | 0.13 | 1.388 | 1.393 | 0.360 | 1.402 | 1.009 | 1.397 | 0.648 |
| 70.0 | 0.15 | 1.440 | 1.446 | 0.417 | 1.458 | 1.250 | 1.453 | 0.903 |
| 80.0 | 0.17 | 1.490 | 1.495 | 0.336 | 1.510 | 1.342 | 1.505 | 1.007 |
| 90.0 | 0.20 | 1.536 | 1.542 | 0.391 | 1.560 | 1.563 | 1.554 | 1.172 |
| 100.0 | 0.22 | 1.582 | 1.586 | 0.253 | 1.607 | 1.580 | 1.601 | 1.201 |
| 110.0 | 0.24 | 1.624 | 1.629 | 0.308 | 1.652 | 1.724 | 1.646 | 1.355 |
| 120.0 | 0.26 | 1.664 | 1.670 | 0.361 | 1.695 | 1.863 | 1.689 | 1.502 |
| 130.0 | 0.28 | 1.702 | 1.710 | 0.470 | 1.736 | 1.998 | 1.731 | 1.704 |
| 140.0 | 0.31 | 1.741 | 1.748 | 0.402 | 1.776 | 2.010 | 1.771 | 1.723 |
| 150.0 | 0.33 | 1.777 | 1.785 | 0.450 | 1.815 | 2.138 | 1.810 | 1.857 |
| 160.0 | 0.35 | 1.812 | 1.821 | 0.497 | 1.852 | 2.208 | 1.848 | 1.987 |
| 170.0 | 0.37 | 1.847 | 1.856 | 0.487 | 1.888 | 2.220 | 1.885 | 2.057 |
| 180.0 | 0.39 | 1.879 | 1.890 | 0.585 | 1.923 | 2.342 | 1.921 | 2.235 |
| 190.0 | 0.41 | 1.912 | 1.923 | 0.575 | 1.958 | 2.406 | 1.957 | 2.354 |
| 200.0 | 0.44 | 1.944 | 1.955 | 0.566 | 1.991 | 2.418 | 1.991 | 2.418 |
| 210.0 | 0.46 | 1.974 | 1.987 | 0.659 | 2.024 | 2.533 | 2.025 | 2.584 |
| 220.0 | 0.48 | 2.004 | 2.017 | 0.649 | 2.055 | 2.545 | 2.057 | 2.645 |
| 230.0 | 0.50 | 2.034 | 2.047 | 0.639 | 2.087 | 2.606 | 2.090 | 2.753 |
| 240.0 | 0.52 | 2.062 | 2.077 | 0.727 | 2.117 | 2.667 | 2.121 | 2.861 |
| 250.0 | 0.55 | 2.091 | 2.106 | 0.717 | 2.147 | 2.678 | 2.152 | 2.917 |
| 260.0 | 0.57 | 2.119 | 2.134 | 0.708 | 2.176 | 2.690 | 2.183 | 3.020 |
| 270.0 | 0.59 | 2.145 | 2.161 | 0.746 | 2.205 | 2.797 | 2.213 | 3.170 |
| 280.0 | 0.61 | 2.173 | 2.189 | 0.736 | 2.233 | 2.761 | 2.243 | 3.221 |
| 290.0 | 0.63 | 2.198 | 2.215 | 0.773 | 2.261 | 2.866 | 2.272 | 3.367 |
| 300.0 | 0.65 | 2.225 | 2.241 | 0.719 | 2.288 | 2.831 | 2.300 | 3.371 |
| 310.0 | 0.68 | 2.250 | 2.267 | 0.756 | 2.315 | 2.889 | 2.328 | 3.467 |
| 320.0 | 0.70 | 2.274 | 2.292 | 0.792 | 2.341 | 2.946 | 2.356 | 3.606 |
| 330.0 | 0.72 | 2.299 | 2.317 | 0.783 | 2.367 | 2.958 | 2.383 | 3.654 |
| 340.0 | 0.74 | 2.324 | 2.342 | 0.775 | 2.393 | 2.969 | 2.410 | 3.701 |
| 350.0 | 0.76 | 2.347 | 2.365 | 0.767 | 2.418 | 3.025 | 2.436 | 3.792 |
| 360.0 | 0.79 | 2.371 | 2.389 | 0.759 | 2.443 | 3.037 | 2.463 | 3.880 |
| 370.0 | 0.81 | 2.394 | 2.412 | 0.752 | 2.468 | 3.091 | 2.488 | 3.926 |
| 380.0 | 0.83 | 2.417 | 2.435 | 0.745 | 2.492 | 3.103 | 2.514 | 4.013 |
| 390.0 | 0.85 | 2.438 | 2.457 | 0.779 | 2.516 | 3.199 | 2.539 | 4.143 |
| 400.0 | 0.87 | 2.462 | 2.479 | 0.690 | 2.539 | 3.128 | 2.563 | 4.102 |
| $\boldsymbol{\epsilon_{\mathrm{AVE}}}(\%)$ | | | | **0.576** | | **2.292** | | **2.450** |
| $\boldsymbol{\epsilon_{\mathrm{MAX}}}(\%)$ | | | | **0.792** | | **3.199** | | **4.143** |

**Table 3a.** Key properties of the radial distribution function as resulting from molecular dynamics (MD) simulations and from three integral equation theory approaches: the updated version of the isomorph-based empirically modified hypernetted chain approximation (IEMHNC) introduced in the present letter, the variational modified hypernetted-chain approximation (VMHNC) discussed in *G. Faussurier, Phys. Rev. E* **69**, *066402 (2004)* and the empirically modified hypernetted-chain approximation (EMHNC) presented in *W. Daughton, M. S. Murillo and L. Thode, Phys. Rev. E* **61**, *2129 (2000)*. The absolute relative deviation $\epsilon_{\mathrm{r}}$ between the theoretical and the simulation results is also reported together with its average and maximum values (the average deviation is denoted as $\epsilon_{\mathrm{AVE}}$ and the maximum deviation is denoted as $\epsilon_{\mathrm{MAX}}$). **Results for the position of the first maximum in the case of $\boldsymbol{\kappa = 0.0}$**. The MD results are adopted from *T. Ott and M. Bonitz, Contrib. Plasma Phys.* **55**, *243 (2015)*. Here $x = r/d$, where $d$ is the Wigner-Seitz radius.

| $\Gamma$ | $\Gamma/\Gamma_m$ | $x_{\mathrm{max1}}^{\mathrm{MD}}$ | $x_{\mathrm{max1}}^{\mathrm{IEMHNC}}$ | $\epsilon_{\mathrm{IEMHNC}}(\%)$ | $x_{\mathrm{max1}}^{\mathrm{VMHNC}}$ | $\epsilon_{\mathrm{VMHNC}}(\%)$ | $x_{\mathrm{max1}}^{\mathrm{EMHNC}}$ | $\epsilon_{\mathrm{EMHNC}}(\%)$ |
|---|---|---|---|---|---|---|---|---|
| 15.0 | 0.09 | 1.666 | 1.660 | 0.360 | 1.644 | 1.321 | 1.678 | 0.720 |
| 20.0 | 0.12 | 1.665 | 1.663 | 0.120 | 1.647 | 1.081 | 1.672 | 0.420 |
| 25.0 | 0.15 | 1.668 | 1.669 | 0.060 | 1.652 | 0.959 | 1.670 | 0.120 |
| 30.0 | 0.17 | 1.671 | 1.674 | 0.180 | 1.658 | 0.778 | 1.670 | 0.060 |
| 35.0 | 0.20 | 1.674 | 1.678 | 0.239 | 1.664 | 0.597 | 1.671 | 0.179 |
| 40.0 | 0.23 | 1.678 | 1.680 | 0.119 | 1.669 | 0.536 | 1.673 | 0.298 |
| 45.0 | 0.26 | 1.681 | 1.683 | 0.119 | 1.674 | 0.416 | 1.676 | 0.297 |
| 50.0 | 0.29 | 1.685 | 1.685 | 0.000 | 1.678 | 0.415 | 1.678 | 0.415 |
| 55.0 | 0.32 | 1.688 | 1.688 | 0.000 | 1.683 | 0.296 | 1.681 | 0.415 |
| 60.0 | 0.35 | 1.690 | 1.690 | 0.000 | 1.687 | 0.178 | 1.683 | 0.414 |
| 65.0 | 0.38 | 1.693 | 1.692 | 0.059 | 1.690 | 0.177 | 1.686 | 0.413 |
| 70.0 | 0.41 | 1.696 | 1.694 | 0.118 | 1.694 | 0.118 | 1.688 | 0.472 |
| 75.0 | 0.44 | 1.698 | 1.697 | 0.059 | 1.697 | 0.059 | 1.690 | 0.471 |
| 80.0 | 0.47 | 1.701 | 1.699 | 0.118 | 1.700 | 0.059 | 1.693 | 0.470 |
| 85.0 | 0.49 | 1.703 | 1.701 | 0.117 | 1.703 | 0.000 | 1.695 | 0.470 |
| 90.0 | 0.52 | 1.705 | 1.703 | 0.117 | 1.705 | 0.000 | 1.697 | 0.469 |
| 95.0 | 0.55 | 1.707 | 1.705 | 0.117 | 1.708 | 0.059 | 1.699 | 0.469 |
| 100.0 | 0.58 | 1.709 | 1.707 | 0.117 | 1.710 | 0.059 | 1.701 | 0.468 |
| 105.0 | 0.61 | 1.710 | 1.709 | 0.058 | 1.713 | 0.175 | 1.703 | 0.409 |
| 110.0 | 0.64 | 1.712 | 1.711 | 0.058 | 1.715 | 0.175 | 1.705 | 0.409 |
| 115.0 | 0.67 | 1.714 | 1.713 | 0.058 | 1.717 | 0.175 | 1.707 | 0.408 |
| 120.0 | 0.70 | 1.715 | 1.715 | 0.000 | 1.719 | 0.233 | 1.708 | 0.408 |
| 125.0 | 0.73 | 1.717 | 1.716 | 0.058 | 1.721 | 0.233 | 1.710 | 0.408 |
| 130.0 | 0.76 | 1.719 | 1.718 | 0.058 | 1.722 | 0.175 | 1.712 | 0.407 |
| 135.0 | 0.79 | 1.720 | 1.719 | 0.058 | 1.724 | 0.233 | 1.713 | 0.407 |
| 140.0 | 0.81 | 1.721 | 1.721 | 0.000 | 1.726 | 0.291 | 1.715 | 0.349 |
| 145.0 | 0.84 | 1.723 | 1.722 | 0.058 | 1.728 | 0.290 | 1.716 | 0.406 |
| 150.0 | 0.87 | 1.724 | 1.724 | 0.000 | 1.729 | 0.290 | 1.718 | 0.348 |
| 155.0 | 0.90 | 1.725 | 1.725 | 0.000 | 1.731 | 0.348 | 1.719 | 0.348 |
| 160.0 | 0.93 | 1.727 | 1.726 | 0.058 | 1.732 | 0.290 | 1.721 | 0.347 |
| $\boldsymbol{\epsilon_{\mathrm{AVE}}}$**(%)** | | | | **0.083** | | **0.334** | | **0.390** |
| $\boldsymbol{\epsilon_{\mathrm{MAX}}}$**(%)** | | | | **0.360** | | **1.321** | | **0.720** |

**Table 3b.** Key properties of the radial distribution function as resulting from molecular dynamics (MD) simulations and from three integral equation theory approaches: the updated version of the isomorph-based empirically modified hypernetted chain approximation (IEMHNC) introduced in the present letter, the variational modified hypernetted-chain approximation (VMHNC) discussed in *G. Faussurier, Phys. Rev. E* **69**, *066402 (2004)* and the empirically modified hypernetted-chain approximation (EMHNC) presented in *W. Daughton, M. S. Murillo and L. Thode, Phys. Rev. E* **61**, *2129 (2000)*. The absolute relative deviation $\epsilon_{\mathrm{r}}$ between the theoretical and the simulation results is also reported together with its average and maximum values (the average deviation is denoted as $\epsilon_{\mathrm{AVE}}$ and the maximum deviation is denoted as $\epsilon_{\mathrm{MAX}}$). **Results for the position of the first maximum in the case of $\boldsymbol{\kappa = 1.0}$**. The MD results are adopted from *T. Ott and M. Bonitz, Contrib. Plasma Phys.* **55**, *243 (2015)*. Here $x = r/d$, where $d$ is the Wigner-Seitz radius.

| $\Gamma$ | $\Gamma/\Gamma_m$ | $x_{\mathrm{max1}}^{\mathrm{MD}}$ | $x_{\mathrm{max1}}^{\mathrm{IEMHNC}}$ | $\epsilon_{\mathrm{IEMHNC}}(\%)$ | $x_{\mathrm{max1}}^{\mathrm{VMHNC}}$ | $\epsilon_{\mathrm{VMHNC}}(\%)$ | $x_{\mathrm{max1}}^{\mathrm{EMHNC}}$ | $\epsilon_{\mathrm{EMHNC}}(\%)$ |
|---|---|---|---|---|---|---|---|---|
| 10.0 | 0.05 | 1.660 | 1.679 | 1.145 | 1.635 | 1.506 | 1.675 | 0.904 |
| 15.0 | 0.07 | 1.648 | 1.645 | 0.182 | 1.624 | 1.456 | 1.662 | 0.850 |
| 20.0 | 0.09 | 1.648 | 1.643 | 0.303 | 1.627 | 1.274 | 1.656 | 0.485 |
| 25.0 | 0.11 | 1.650 | 1.649 | 0.061 | 1.632 | 1.091 | 1.655 | 0.303 |
| 30.0 | 0.14 | 1.655 | 1.655 | 0.000 | 1.638 | 1.027 | 1.656 | 0.060 |
| 35.0 | 0.16 | 1.659 | 1.661 | 0.121 | 1.644 | 0.904 | 1.657 | 0.121 |
| 40.0 | 0.18 | 1.662 | 1.665 | 0.181 | 1.650 | 0.722 | 1.660 | 0.120 |
| 45.0 | 0.20 | 1.666 | 1.669 | 0.180 | 1.655 | 0.660 | 1.662 | 0.240 |
| 50.0 | 0.23 | 1.669 | 1.672 | 0.180 | 1.660 | 0.539 | 1.665 | 0.240 |
| 55.0 | 0.25 | 1.673 | 1.675 | 0.120 | 1.664 | 0.538 | 1.668 | 0.299 |
| 60.0 | 0.27 | 1.676 | 1.677 | 0.060 | 1.668 | 0.477 | 1.670 | 0.358 |
| 65.0 | 0.30 | 1.679 | 1.679 | 0.000 | 1.672 | 0.417 | 1.673 | 0.357 |
| 70.0 | 0.32 | 1.681 | 1.681 | 0.000 | 1.676 | 0.297 | 1.675 | 0.357 |
| 75.0 | 0.34 | 1.684 | 1.683 | 0.059 | 1.679 | 0.297 | 1.678 | 0.356 |
| 80.0 | 0.36 | 1.687 | 1.685 | 0.119 | 1.682 | 0.296 | 1.680 | 0.415 |
| 85.0 | 0.39 | 1.689 | 1.687 | 0.118 | 1.685 | 0.237 | 1.683 | 0.355 |
| 90.0 | 0.41 | 1.691 | 1.689 | 0.118 | 1.688 | 0.177 | 1.685 | 0.355 |
| 95.0 | 0.43 | 1.693 | 1.691 | 0.118 | 1.691 | 0.118 | 1.687 | 0.354 |
| 100.0 | 0.45 | 1.695 | 1.693 | 0.118 | 1.694 | 0.059 | 1.689 | 0.354 |
| 105.0 | 0.48 | 1.697 | 1.695 | 0.118 | 1.696 | 0.059 | 1.691 | 0.354 |
| 110.0 | 0.50 | 1.699 | 1.697 | 0.118 | 1.698 | 0.059 | 1.693 | 0.353 |
| 115.0 | 0.52 | 1.701 | 1.699 | 0.118 | 1.701 | 0.000 | 1.695 | 0.353 |
| 120.0 | 0.54 | 1.702 | 1.701 | 0.059 | 1.703 | 0.059 | 1.697 | 0.294 |
| 125.0 | 0.57 | 1.704 | 1.702 | 0.117 | 1.705 | 0.059 | 1.699 | 0.293 |
| 130.0 | 0.59 | 1.706 | 1.704 | 0.117 | 1.707 | 0.059 | 1.700 | 0.352 |
| 135.0 | 0.61 | 1.707 | 1.706 | 0.059 | 1.709 | 0.117 | 1.702 | 0.293 |
| 140.0 | 0.64 | 1.709 | 1.707 | 0.117 | 1.710 | 0.059 | 1.704 | 0.293 |
| 145.0 | 0.66 | 1.710 | 1.709 | 0.058 | 1.712 | 0.117 | 1.705 | 0.292 |
| 150.0 | 0.68 | 1.712 | 1.710 | 0.117 | 1.714 | 0.117 | 1.707 | 0.292 |
| 155.0 | 0.70 | 1.713 | 1.712 | 0.058 | 1.715 | 0.117 | 1.708 | 0.292 |
| 160.0 | 0.73 | 1.715 | 1.713 | 0.117 | 1.717 | 0.117 | 1.710 | 0.292 |
| 165.0 | 0.75 | 1.715 | 1.714 | 0.058 | 1.718 | 0.175 | 1.711 | 0.233 |
| 170.0 | 0.77 | 1.717 | 1.716 | 0.058 | 1.720 | 0.175 | 1.713 | 0.233 |
| 175.0 | 0.79 | 1.718 | 1.717 | 0.058 | 1.721 | 0.175 | 1.714 | 0.233 |
| 180.0 | 0.82 | 1.719 | 1.718 | 0.058 | 1.723 | 0.233 | 1.715 | 0.233 |
| 185.0 | 0.84 | 1.720 | 1.719 | 0.058 | 1.724 | 0.233 | 1.717 | 0.174 |
| 190.0 | 0.86 | 1.721 | 1.720 | 0.058 | 1.725 | 0.232 | 1.718 | 0.174 |
| 195.0 | 0.89 | 1.722 | 1.722 | 0.000 | 1.727 | 0.290 | 1.719 | 0.174 |
| 200.0 | 0.91 | 1.723 | 1.723 | 0.000 | 1.728 | 0.290 | 1.720 | 0.174 |
| $\boldsymbol{\epsilon_{\mathrm{AVE}}}(\%)$ | | | | **0.121** | | **0.380** | | **0.314** |
| $\boldsymbol{\epsilon_{\mathrm{MAX}}}(\%)$ | | | | **1.145** | | **1.506** | | **0.904** |

**Table 3c.** Key properties of the radial distribution function as resulting from molecular dynamics (MD) simulations and from three integral equation theory approaches: the updated version of the isomorph-based empirically modified hypernetted chain approximation (IEMHNC) introduced in the present letter, the variational modified hypernetted-chain approximation (VMHNC) discussed in *G. Faussurier, Phys. Rev. E* **69**, *066402 (2004)* and the empirically modified hypernetted-chain approximation (EMHNC) presented in *W. Daughton, M. S. Murillo and L. Thode, Phys. Rev. E* **61**, *2129 (2000)*. The absolute relative deviation $\epsilon_{\rm r}$ between the theoretical and the simulation results is also reported together with its average and maximum values (the average deviation is denoted as $\epsilon_{\rm AVE}$ and the maximum deviation is denoted as $\epsilon_{\rm MAX}$). **Results for the position of the first maximum in the case of $\boldsymbol{\kappa = 2.0}$**. The MD results are adopted from *T. Ott and M. Bonitz, Contrib. Plasma Phys.* **55**, *243 (2015)*. Here $x = r/d$, where $d$ is the Wigner-Seitz radius.

| $\Gamma$ | $\Gamma/\Gamma_m$ | $x_{\rm max1}^{\rm MD}$ | $x_{\rm max1}^{\rm IEMHNC}$ | $\epsilon_{\rm IEMHNC}(\%)$ | $x_{\rm max1}^{\rm VMHNC}$ | $\epsilon_{\rm VMHNC}(\%)$ | $x_{\rm max1}^{\rm EMHNC}$ | $\epsilon_{\rm EMHNC}(\%)$ |
|---|---|---|---|---|---|---|---|---|
| 30.0 | 0.07 | 1.598 | 1.597 | 0.063 | 1.580 | 1.126 | 1.609 | 0.688 |
| 40.0 | 0.09 | 1.609 | 1.605 | 0.249 | 1.592 | 1.057 | 1.615 | 0.373 |
| 50.0 | 0.11 | 1.619 | 1.616 | 0.185 | 1.603 | 0.988 | 1.622 | 0.185 |
| 60.0 | 0.13 | 1.627 | 1.627 | 0.000 | 1.613 | 0.860 | 1.629 | 0.123 |
| 70.0 | 0.15 | 1.633 | 1.635 | 0.122 | 1.621 | 0.735 | 1.635 | 0.122 |
| 80.0 | 0.17 | 1.640 | 1.642 | 0.122 | 1.629 | 0.671 | 1.640 | 0.000 |
| 90.0 | 0.20 | 1.646 | 1.648 | 0.122 | 1.636 | 0.608 | 1.645 | 0.061 |
| 100.0 | 0.22 | 1.651 | 1.652 | 0.061 | 1.642 | 0.545 | 1.650 | 0.061 |
| 110.0 | 0.24 | 1.656 | 1.656 | 0.000 | 1.647 | 0.543 | 1.655 | 0.060 |
| 120.0 | 0.26 | 1.660 | 1.660 | 0.000 | 1.653 | 0.422 | 1.659 | 0.060 |
| 130.0 | 0.28 | 1.664 | 1.663 | 0.060 | 1.657 | 0.421 | 1.663 | 0.060 |
| 140.0 | 0.31 | 1.668 | 1.666 | 0.120 | 1.662 | 0.360 | 1.667 | 0.060 |
| 150.0 | 0.33 | 1.671 | 1.669 | 0.120 | 1.666 | 0.299 | 1.671 | 0.000 |
| 160.0 | 0.35 | 1.674 | 1.672 | 0.119 | 1.670 | 0.239 | 1.674 | 0.000 |
| 170.0 | 0.37 | 1.677 | 1.674 | 0.179 | 1.673 | 0.239 | 1.677 | 0.000 |
| 180.0 | 0.39 | 1.680 | 1.677 | 0.179 | 1.676 | 0.238 | 1.680 | 0.000 |
| 190.0 | 0.41 | 1.683 | 1.679 | 0.238 | 1.680 | 0.178 | 1.683 | 0.000 |
| 200.0 | 0.44 | 1.685 | 1.681 | 0.237 | 1.682 | 0.178 | 1.686 | 0.059 |
| 210.0 | 0.46 | 1.687 | 1.684 | 0.178 | 1.685 | 0.119 | 1.689 | 0.119 |
| 220.0 | 0.48 | 1.690 | 1.686 | 0.237 | 1.688 | 0.118 | 1.691 | 0.059 |
| 230.0 | 0.50 | 1.691 | 1.688 | 0.177 | 1.691 | 0.000 | 1.694 | 0.177 |
| 240.0 | 0.52 | 1.693 | 1.690 | 0.177 | 1.693 | 0.000 | 1.696 | 0.177 |
| 250.0 | 0.55 | 1.696 | 1.692 | 0.236 | 1.695 | 0.059 | 1.698 | 0.118 |
| 260.0 | 0.57 | 1.698 | 1.694 | 0.236 | 1.697 | 0.059 | 1.701 | 0.177 |
| 270.0 | 0.59 | 1.699 | 1.696 | 0.177 | 1.700 | 0.059 | 1.703 | 0.235 |
| 280.0 | 0.61 | 1.701 | 1.698 | 0.176 | 1.702 | 0.059 | 1.705 | 0.235 |
| 290.0 | 0.63 | 1.703 | 1.700 | 0.176 | 1.704 | 0.059 | 1.707 | 0.235 |
| 300.0 | 0.65 | 1.704 | 1.701 | 0.176 | 1.705 | 0.059 | 1.709 | 0.293 |
| 310.0 | 0.68 | 1.706 | 1.703 | 0.176 | 1.707 | 0.059 | 1.710 | 0.234 |
| 320.0 | 0.70 | 1.708 | 1.704 | 0.234 | 1.709 | 0.059 | 1.712 | 0.234 |
| 330.0 | 0.72 | 1.709 | 1.706 | 0.176 | 1.711 | 0.117 | 1.714 | 0.293 |
| 340.0 | 0.74 | 1.711 | 1.707 | 0.234 | 1.712 | 0.058 | 1.716 | 0.292 |
| 350.0 | 0.76 | 1.712 | 1.709 | 0.175 | 1.714 | 0.117 | 1.717 | 0.292 |
| 360.0 | 0.79 | 1.713 | 1.710 | 0.175 | 1.715 | 0.117 | 1.719 | 0.350 |
| 370.0 | 0.81 | 1.715 | 1.712 | 0.175 | 1.717 | 0.117 | 1.720 | 0.292 |
| 380.0 | 0.83 | 1.716 | 1.713 | 0.175 | 1.718 | 0.117 | 1.722 | 0.350 |
| 390.0 | 0.85 | 1.717 | 1.714 | 0.175 | 1.720 | 0.175 | 1.723 | 0.349 |
| 400.0 | 0.87 | 1.718 | 1.715 | 0.175 | 1.721 | 0.175 | 1.724 | 0.349 |
| $\boldsymbol{\epsilon_{\rm AVE}}(\%)$ | | | | **0.158** | | **0.300** | | **0.178** |
| $\boldsymbol{\epsilon_{\rm MAX}}(\%)$ | | | | **0.249** | | **1.126** | | **0.688** |

**Table 4a.** Key properties of the radial distribution function as resulting from molecular dynamics (MD) simulations and from three integral equation theory approaches: the updated version of the isomorph-based empirically modified hypernetted chain approximation (IEMHNC) introduced in the present letter, the variational modified hypernetted-chain approximation (VMHNC) discussed in *G. Faussurier, Phys. Rev. E* **69**, *066402 (2004)* and the empirically modified hypernetted-chain approximation (EMHNC) presented in *W. Daughton, M. S. Murillo and L. Thode, Phys. Rev. E* **61**, *2129 (2000)*. The absolute relative deviation $\epsilon_{\mathrm{r}}$ between the theoretical and the simulation results is also reported together with its average and maximum values (the average deviation is denoted as $\epsilon_{\mathrm{AVE}}$ and the maximum deviation is denoted as $\epsilon_{\mathrm{MAX}}$). **Results for the magnitude of the first non-zero minimum in the case of $\boldsymbol{\kappa = 0.0}$**. The MD results are adopted from *T. Ott and M. Bonitz, Contrib. Plasma Phys.* **55**, *243 (2015)*.

| $\Gamma$ | $\Gamma/\Gamma_m$ | $g_{\mathrm{min1}}^{\mathrm{MD}}$ | $g_{\mathrm{min1}}^{\mathrm{IEMHNC}}$ | $\epsilon_{\mathrm{IEMHNC}}(\%)$ | $g_{\mathrm{min1}}^{\mathrm{VMHNC}}$ | $\epsilon_{\mathrm{VMHNC}}(\%)$ | $g_{\mathrm{min1}}^{\mathrm{EMHNC}}$ | $\epsilon_{\mathrm{EMHNC}}(\%)$ |
|---|---|---|---|---|---|---|---|---|
| 15.0 | 0.09 | 1.228 | 1.227 | 0.081 | 1.228 | 0.000 | 1.200 | 2.280 |
| 20.0 | 0.12 | 1.307 | 1.307 | 0.000 | 1.312 | 0.383 | 1.277 | 2.295 |
| 25.0 | 0.15 | 1.378 | 1.378 | 0.000 | 1.387 | 0.653 | 1.348 | 2.177 |
| 30.0 | 0.17 | 1.443 | 1.442 | 0.069 | 1.457 | 0.970 | 1.414 | 2.010 |
| 35.0 | 0.20 | 1.504 | 1.502 | 0.133 | 1.521 | 1.130 | 1.475 | 1.928 |
| 40.0 | 0.23 | 1.560 | 1.557 | 0.192 | 1.581 | 1.346 | 1.533 | 1.731 |
| 45.0 | 0.26 | 1.614 | 1.610 | 0.248 | 1.637 | 1.425 | 1.587 | 1.673 |
| 50.0 | 0.29 | 1.664 | 1.661 | 0.180 | 1.691 | 1.623 | 1.639 | 1.502 |
| 55.0 | 0.32 | 1.712 | 1.709 | 0.175 | 1.741 | 1.694 | 1.688 | 1.402 |
| 60.0 | 0.35 | 1.757 | 1.755 | 0.114 | 1.790 | 1.878 | 1.735 | 1.252 |
| 65.0 | 0.38 | 1.803 | 1.799 | 0.222 | 1.837 | 1.886 | 1.781 | 1.220 |
| 70.0 | 0.41 | 1.845 | 1.842 | 0.163 | 1.881 | 1.951 | 1.824 | 1.138 |
| 75.0 | 0.44 | 1.885 | 1.884 | 0.053 | 1.925 | 2.122 | 1.867 | 0.955 |
| 80.0 | 0.47 | 1.926 | 1.924 | 0.104 | 1.966 | 2.077 | 1.908 | 0.935 |
| 85.0 | 0.49 | 1.964 | 1.963 | 0.051 | 2.007 | 2.189 | 1.948 | 0.815 |
| 90.0 | 0.52 | 2.001 | 2.001 | 0.000 | 2.046 | 2.249 | 1.987 | 0.700 |
| 95.0 | 0.55 | 2.037 | 2.037 | 0.000 | 2.084 | 2.307 | 2.025 | 0.589 |
| 100.0 | 0.58 | 2.072 | 2.073 | 0.048 | 2.122 | 2.413 | 2.063 | 0.434 |
| 105.0 | 0.61 | 2.107 | 2.108 | 0.047 | 2.158 | 2.421 | 2.099 | 0.380 |
| 110.0 | 0.64 | 2.140 | 2.143 | 0.140 | 2.193 | 2.477 | 2.134 | 0.280 |
| 115.0 | 0.67 | 2.174 | 2.176 | 0.092 | 2.228 | 2.484 | 2.169 | 0.230 |
| 120.0 | 0.70 | 2.206 | 2.209 | 0.136 | 2.262 | 2.539 | 2.204 | 0.091 |
| 125.0 | 0.73 | 2.237 | 2.240 | 0.134 | 2.295 | 2.593 | 2.237 | 0.000 |
| 130.0 | 0.76 | 2.270 | 2.271 | 0.044 | 2.327 | 2.511 | 2.270 | 0.000 |
| 135.0 | 0.79 | 2.298 | 2.302 | 0.174 | 2.359 | 2.654 | 2.303 | 0.218 |
| 140.0 | 0.81 | 2.329 | 2.331 | 0.086 | 2.390 | 2.619 | 2.334 | 0.215 |
| 145.0 | 0.84 | 2.358 | 2.360 | 0.085 | 2.421 | 2.672 | 2.366 | 0.339 |
| 150.0 | 0.87 | 2.386 | 2.388 | 0.084 | 2.451 | 2.724 | 2.397 | 0.461 |
| 155.0 | 0.90 | 2.413 | 2.416 | 0.124 | 2.481 | 2.818 | 2.427 | 0.580 |
| 160.0 | 0.93 | 2.442 | 2.442 | 0.000 | 2.510 | 2.785 | 2.457 | 0.614 |
| $\boldsymbol{\epsilon_{\mathrm{AVE}}}(\%)$ | | | | **0.099** | | **1.986** | | **0.948** |
| $\boldsymbol{\epsilon_{\mathrm{MAX}}}(\%)$ | | | | **0.248** | | **2.818** | | **2.295** |

**Table 4b.** Key properties of the radial distribution function as resulting from molecular dynamics (MD) simulations and from three integral equation theory approaches: the updated version of the isomorph-based empirically modified hypernetted chain approximation (IEMHNC) introduced in the present letter, the variational modified hypernetted-chain approximation (VMHNC) discussed in *G. Faussurier, Phys. Rev. E* **69**, *066402 (2004)* and the empirically modified hypernetted-chain approximation (EMHNC) presented in *W. Daughton, M. S. Murillo and L. Thode, Phys. Rev. E* **61**, *2129 (2000)*. The absolute relative deviation $\epsilon_{\mathrm{r}}$ between the theoretical and the simulation results is also reported together with its average and maximum values (the average deviation is denoted as $\epsilon_{\mathrm{AVE}}$ and the maximum deviation is denoted as $\epsilon_{\mathrm{MAX}}$). **Results for the magnitude of the first non-zero minimum in the case of $\boldsymbol{\kappa = 1.0}$.** The MD results are adopted from *T. Ott and M. Bonitz, Contrib. Plasma Phys.* **55**, *243 (2015)*.

| $\Gamma$ | $\Gamma/\Gamma_m$ | $g_{\mathrm{min1}}^{\mathrm{MD}}$ | $g_{\mathrm{min1}}^{\mathrm{IEMHNC}}$ | $\epsilon_{\mathrm{IEMHNC}}(\%)$ | $g_{\mathrm{min1}}^{\mathrm{VMHNC}}$ | $\epsilon_{\mathrm{VMHNC}}(\%)$ | $g_{\mathrm{min1}}^{\mathrm{EMHNC}}$ | $\epsilon_{\mathrm{EMHNC}}(\%)$ |
|---|---|---|---|---|---|---|---|---|
| 10.0 | 0.05 | 1.101 | 1.100 | 0.091 | 1.097 | 0.363 | 1.089 | 1.090 |
| 15.0 | 0.07 | 1.175 | 1.176 | 0.085 | 1.174 | 0.085 | 1.159 | 1.362 |
| 20.0 | 0.09 | 1.243 | 1.246 | 0.241 | 1.245 | 0.161 | 1.225 | 1.448 |
| 25.0 | 0.11 | 1.304 | 1.309 | 0.383 | 1.310 | 0.460 | 1.288 | 1.227 |
| 30.0 | 0.14 | 1.360 | 1.365 | 0.368 | 1.370 | 0.735 | 1.345 | 1.103 |
| 35.0 | 0.16 | 1.413 | 1.418 | 0.354 | 1.426 | 0.920 | 1.400 | 0.920 |
| 40.0 | 0.18 | 1.462 | 1.466 | 0.274 | 1.478 | 1.094 | 1.450 | 0.821 |
| 45.0 | 0.20 | 1.509 | 1.513 | 0.265 | 1.528 | 1.259 | 1.499 | 0.663 |
| 50.0 | 0.23 | 1.553 | 1.557 | 0.258 | 1.575 | 1.417 | 1.544 | 0.580 |
| 55.0 | 0.25 | 1.595 | 1.599 | 0.251 | 1.619 | 1.505 | 1.588 | 0.439 |
| 60.0 | 0.27 | 1.636 | 1.640 | 0.244 | 1.662 | 1.589 | 1.630 | 0.367 |
| 65.0 | 0.30 | 1.675 | 1.679 | 0.239 | 1.704 | 1.731 | 1.670 | 0.299 |
| 70.0 | 0.32 | 1.711 | 1.717 | 0.351 | 1.743 | 1.870 | 1.709 | 0.117 |
| 75.0 | 0.34 | 1.749 | 1.753 | 0.229 | 1.781 | 1.830 | 1.747 | 0.114 |
| 80.0 | 0.36 | 1.783 | 1.789 | 0.337 | 1.818 | 1.963 | 1.784 | 0.056 |
| 85.0 | 0.39 | 1.817 | 1.823 | 0.330 | 1.854 | 2.036 | 1.819 | 0.110 |
| 90.0 | 0.41 | 1.850 | 1.857 | 0.378 | 1.889 | 2.108 | 1.854 | 0.216 |
| 95.0 | 0.43 | 1.882 | 1.890 | 0.425 | 1.923 | 2.179 | 1.888 | 0.319 |
| 100.0 | 0.45 | 1.914 | 1.921 | 0.366 | 1.956 | 2.194 | 1.921 | 0.366 |
| 105.0 | 0.48 | 1.944 | 1.953 | 0.463 | 1.988 | 2.263 | 1.953 | 0.463 |
| 110.0 | 0.50 | 1.974 | 1.983 | 0.456 | 2.020 | 2.330 | 1.985 | 0.557 |
| 115.0 | 0.52 | 2.003 | 2.013 | 0.499 | 2.051 | 2.396 | 2.016 | 0.649 |
| 120.0 | 0.54 | 2.031 | 2.042 | 0.542 | 2.081 | 2.462 | 2.046 | 0.739 |
| 125.0 | 0.57 | 2.058 | 2.070 | 0.583 | 2.110 | 2.527 | 2.076 | 0.875 |
| 130.0 | 0.59 | 2.088 | 2.098 | 0.479 | 2.139 | 2.443 | 2.106 | 0.862 |
| 135.0 | 0.61 | 2.114 | 2.126 | 0.568 | 2.167 | 2.507 | 2.134 | 0.946 |
| 140.0 | 0.64 | 2.141 | 2.153 | 0.560 | 2.195 | 2.522 | 2.163 | 1.028 |
| 145.0 | 0.66 | 2.166 | 2.179 | 0.600 | 2.222 | 2.585 | 2.191 | 1.154 |
| 150.0 | 0.68 | 2.191 | 2.205 | 0.639 | 2.249 | 2.647 | 2.218 | 1.232 |
| 155.0 | 0.70 | 2.217 | 2.230 | 0.586 | 2.276 | 2.661 | 2.245 | 1.263 |
| 160.0 | 0.73 | 2.242 | 2.255 | 0.580 | 2.302 | 2.676 | 2.272 | 1.338 |
| 165.0 | 0.75 | 2.266 | 2.280 | 0.618 | 2.327 | 2.692 | 2.299 | 1.456 |
| 170.0 | 0.77 | 2.289 | 2.304 | 0.655 | 2.352 | 2.752 | 2.325 | 1.573 |
| 175.0 | 0.79 | 2.314 | 2.327 | 0.562 | 2.377 | 2.723 | 2.350 | 1.556 |
| 180.0 | 0.82 | 2.337 | 2.350 | 0.556 | 2.402 | 2.781 | 2.376 | 1.669 |
| 185.0 | 0.84 | 2.359 | 2.373 | 0.593 | 2.426 | 2.840 | 2.401 | 1.780 |
| 190.0 | 0.86 | 2.383 | 2.395 | 0.504 | 2.450 | 2.812 | 2.425 | 1.762 |
| 195.0 | 0.89 | 2.404 | 2.417 | 0.541 | 2.473 | 2.870 | 2.450 | 1.913 |
| 200.0 | 0.91 | 2.427 | 2.439 | 0.494 | 2.496 | 2.843 | 2.474 | 1.937 |
| $\boldsymbol{\epsilon_{\mathrm{AVE}}}(\%)$ | | | | **0.424** | | **1.996** | | **0.932** |
| $\boldsymbol{\epsilon_{\mathrm{MAX}}}(\%)$ | | | | **0.655** | | **2.870** | | **1.937** |

**Table 4c.** Key properties of the radial distribution function as resulting from molecular dynamics (MD) simulations and from three integral equation theory approaches: the updated version of the isomorph-based empirically modified hypernetted chain approximation (IEMHNC) introduced in the present letter, the variational modified hypernetted-chain approximation (VMHNC) discussed in *G. Faussurier, Phys. Rev. E* **69**, *066402 (2004)* and the empirically modified hypernetted-chain approximation (EMHNC) presented in *W. Daughton, M. S. Murillo and L. Thode, Phys. Rev. E* **61**, *2129 (2000)*. The absolute relative deviation $\epsilon_{\mathrm{r}}$ between the theoretical and the simulation results is also reported together with its average and maximum values (the average deviation is denoted as $\epsilon_{\mathrm{AVE}}$ and the maximum deviation is denoted as $\epsilon_{\mathrm{MAX}}$). **Results for the magnitude of the first non-zero minimum in the case of $\boldsymbol{\kappa = 2.0}$**. The MD results are adopted from *T. Ott and M. Bonitz, Contrib. Plasma Phys.* **55**, *243 (2015)*.

| $\Gamma$ | $\Gamma/\Gamma_m$ | $g_{\mathrm{min1}}^{\mathrm{MD}}$ | $g_{\mathrm{min1}}^{\mathrm{IEMHNC}}$ | $\epsilon_{\mathrm{IEMHNC}}(\%)$ | $g_{\mathrm{min1}}^{\mathrm{VMHNC}}$ | $\epsilon_{\mathrm{VMHNC}}(\%)$ | $g_{\mathrm{min1}}^{\mathrm{EMHNC}}$ | $\epsilon_{\mathrm{EMHNC}}(\%)$ |
|---|---|---|---|---|---|---|---|---|
| 30.0 | 0.07 | 1.202 | 1.202 | 0.000 | 1.206 | 0.333 | 1.201 | 0.083 |
| 40.0 | 0.09 | 1.270 | 1.274 | 0.315 | 1.277 | 0.551 | 1.273 | 0.236 |
| 50.0 | 0.11 | 1.331 | 1.337 | 0.451 | 1.342 | 0.826 | 1.337 | 0.451 |
| 60.0 | 0.13 | 1.388 | 1.393 | 0.360 | 1.402 | 1.009 | 1.397 | 0.648 |
| 70.0 | 0.15 | 1.440 | 1.446 | 0.417 | 1.458 | 1.250 | 1.453 | 0.903 |
| 80.0 | 0.17 | 1.490 | 1.495 | 0.336 | 1.510 | 1.342 | 1.505 | 1.007 |
| 90.0 | 0.20 | 1.536 | 1.542 | 0.391 | 1.560 | 1.563 | 1.554 | 1.172 |
| 100.0 | 0.22 | 1.582 | 1.586 | 0.253 | 1.607 | 1.580 | 1.601 | 1.201 |
| 110.0 | 0.24 | 1.624 | 1.629 | 0.308 | 1.652 | 1.724 | 1.646 | 1.355 |
| 120.0 | 0.26 | 1.664 | 1.670 | 0.361 | 1.695 | 1.863 | 1.689 | 1.502 |
| 130.0 | 0.28 | 1.702 | 1.710 | 0.470 | 1.736 | 1.998 | 1.731 | 1.704 |
| 140.0 | 0.31 | 1.741 | 1.748 | 0.402 | 1.776 | 2.010 | 1.771 | 1.723 |
| 150.0 | 0.33 | 1.777 | 1.785 | 0.450 | 1.815 | 2.138 | 1.810 | 1.857 |
| 160.0 | 0.35 | 1.812 | 1.821 | 0.497 | 1.852 | 2.208 | 1.848 | 1.987 |
| 170.0 | 0.37 | 1.847 | 1.856 | 0.487 | 1.888 | 2.220 | 1.885 | 2.057 |
| 180.0 | 0.39 | 1.879 | 1.890 | 0.585 | 1.923 | 2.342 | 1.921 | 2.235 |
| 190.0 | 0.41 | 1.912 | 1.923 | 0.575 | 1.958 | 2.406 | 1.957 | 2.354 |
| 200.0 | 0.44 | 1.944 | 1.955 | 0.566 | 1.991 | 2.418 | 1.991 | 2.418 |
| 210.0 | 0.46 | 1.974 | 1.987 | 0.659 | 2.024 | 2.533 | 2.025 | 2.584 |
| 220.0 | 0.48 | 2.004 | 2.017 | 0.649 | 2.055 | 2.545 | 2.057 | 2.645 |
| 230.0 | 0.50 | 2.034 | 2.047 | 0.639 | 2.087 | 2.606 | 2.090 | 2.753 |
| 240.0 | 0.52 | 2.062 | 2.077 | 0.727 | 2.117 | 2.667 | 2.121 | 2.861 |
| 250.0 | 0.55 | 2.091 | 2.106 | 0.717 | 2.147 | 2.678 | 2.152 | 2.917 |
| 260.0 | 0.57 | 2.119 | 2.134 | 0.708 | 2.176 | 2.690 | 2.183 | 3.020 |
| 270.0 | 0.59 | 2.145 | 2.161 | 0.746 | 2.205 | 2.797 | 2.213 | 3.170 |
| 280.0 | 0.61 | 2.173 | 2.189 | 0.736 | 2.233 | 2.761 | 2.243 | 3.221 |
| 290.0 | 0.63 | 2.198 | 2.215 | 0.773 | 2.261 | 2.866 | 2.272 | 3.367 |
| 300.0 | 0.65 | 2.225 | 2.241 | 0.719 | 2.288 | 2.831 | 2.300 | 3.371 |
| 310.0 | 0.68 | 2.250 | 2.267 | 0.756 | 2.315 | 2.889 | 2.328 | 3.467 |
| 320.0 | 0.70 | 2.274 | 2.292 | 0.792 | 2.341 | 2.946 | 2.356 | 3.606 |
| 330.0 | 0.72 | 2.299 | 2.317 | 0.783 | 2.367 | 2.958 | 2.383 | 3.654 |
| 340.0 | 0.74 | 2.324 | 2.342 | 0.775 | 2.393 | 2.969 | 2.410 | 3.701 |
| 350.0 | 0.76 | 2.347 | 2.365 | 0.767 | 2.418 | 3.025 | 2.436 | 3.792 |
| 360.0 | 0.79 | 2.371 | 2.389 | 0.759 | 2.443 | 3.037 | 2.463 | 3.880 |
| 370.0 | 0.81 | 2.394 | 2.412 | 0.752 | 2.468 | 3.091 | 2.488 | 3.926 |
| 380.0 | 0.83 | 2.417 | 2.435 | 0.745 | 2.492 | 3.103 | 2.514 | 4.013 |
| 390.0 | 0.85 | 2.438 | 2.457 | 0.779 | 2.516 | 3.199 | 2.539 | 4.143 |
| 400.0 | 0.87 | 2.462 | 2.479 | 0.690 | 2.539 | 3.128 | 2.563 | 4.102 |
| $\boldsymbol{\epsilon_{\mathrm{AVE}}}(\%)$ | | | | **0.576** | | **2.292** | | **2.450** |
| $\boldsymbol{\epsilon_{\mathrm{MAX}}}(\%)$ | | | | **0.792** | | **3.199** | | **4.143** |

**Table 5a.** Key properties of the radial distribution function as resulting from molecular dynamics (MD) simulations and from three integral equation theory approaches: the updated version of the isomorph-based empirically modified hypernetted chain approximation (IEMHNC) introduced in the present letter, the variational modified hypernetted-chain approximation (VMHNC) discussed in *G. Faussurier, Phys. Rev. E* **69***, 066402 (2004)* and the empirically modified hypernetted-chain approximation (EMHNC) presented in *W. Daughton, M. S. Murillo and L. Thode, Phys. Rev. E* **61***, 2129 (2000)*. The absolute relative deviation $\epsilon_{\mathrm{r}}$ between the theoretical and the simulation results is also reported together with its average and maximum values (the average deviation is denoted as $\epsilon_{\mathrm{AVE}}$ and the maximum deviation is denoted as $\epsilon_{\mathrm{MAX}}$). **Results for the position of the first non-zero minimum in the case of $\boldsymbol{\kappa = 0.0}$**. The MD results are adopted from *T. Ott and M. Bonitz, Contrib. Plasma Phys.* **55***, 243 (2015)*. Here $x = r/d$, where $d$ is the Wigner-Seitz radius.

| $\Gamma$ | $\Gamma/\Gamma_m$ | $x_{\mathrm{min1}}^{\mathrm{MD}}$ | $x_{\mathrm{min1}}^{\mathrm{IEMHNC}}$ | $\epsilon_{\mathrm{IEMHNC}}(\%)$ | $x_{\mathrm{min1}}^{\mathrm{VMHNC}}$ | $\epsilon_{\mathrm{VMHNC}}(\%)$ | $x_{\mathrm{min1}}^{\mathrm{EMHNC}}$ | $\epsilon_{\mathrm{EMHNC}}(\%)$ |
|---|---|---|---|---|---|---|---|---|
| 15.0 | 0.09 | 1.666 | 1.660 | 0.360 | 1.644 | 1.321 | 1.678 | 0.720 |
| 20.0 | 0.12 | 1.665 | 1.663 | 0.120 | 1.647 | 1.081 | 1.672 | 0.420 |
| 25.0 | 0.15 | 1.668 | 1.669 | 0.060 | 1.652 | 0.959 | 1.670 | 0.120 |
| 30.0 | 0.17 | 1.671 | 1.674 | 0.180 | 1.658 | 0.778 | 1.670 | 0.060 |
| 35.0 | 0.20 | 1.674 | 1.678 | 0.239 | 1.664 | 0.597 | 1.671 | 0.179 |
| 40.0 | 0.23 | 1.678 | 1.680 | 0.119 | 1.669 | 0.536 | 1.673 | 0.298 |
| 45.0 | 0.26 | 1.681 | 1.683 | 0.119 | 1.674 | 0.416 | 1.676 | 0.297 |
| 50.0 | 0.29 | 1.685 | 1.685 | 0.000 | 1.678 | 0.415 | 1.678 | 0.415 |
| 55.0 | 0.32 | 1.688 | 1.688 | 0.000 | 1.683 | 0.296 | 1.681 | 0.415 |
| 60.0 | 0.35 | 1.690 | 1.690 | 0.000 | 1.687 | 0.178 | 1.683 | 0.414 |
| 65.0 | 0.38 | 1.693 | 1.692 | 0.059 | 1.690 | 0.177 | 1.686 | 0.413 |
| 70.0 | 0.41 | 1.696 | 1.694 | 0.118 | 1.694 | 0.118 | 1.688 | 0.472 |
| 75.0 | 0.44 | 1.698 | 1.697 | 0.059 | 1.697 | 0.059 | 1.690 | 0.471 |
| 80.0 | 0.47 | 1.701 | 1.699 | 0.118 | 1.700 | 0.059 | 1.693 | 0.470 |
| 85.0 | 0.49 | 1.703 | 1.701 | 0.117 | 1.703 | 0.000 | 1.695 | 0.470 |
| 90.0 | 0.52 | 1.705 | 1.703 | 0.117 | 1.705 | 0.000 | 1.697 | 0.469 |
| 95.0 | 0.55 | 1.707 | 1.705 | 0.117 | 1.708 | 0.059 | 1.699 | 0.469 |
| 100.0 | 0.58 | 1.709 | 1.707 | 0.117 | 1.710 | 0.059 | 1.701 | 0.468 |
| 105.0 | 0.61 | 1.710 | 1.709 | 0.058 | 1.713 | 0.175 | 1.703 | 0.409 |
| 110.0 | 0.64 | 1.712 | 1.711 | 0.058 | 1.715 | 0.175 | 1.705 | 0.409 |
| 115.0 | 0.67 | 1.714 | 1.713 | 0.058 | 1.717 | 0.175 | 1.707 | 0.408 |
| 120.0 | 0.70 | 1.715 | 1.715 | 0.000 | 1.719 | 0.233 | 1.708 | 0.408 |
| 125.0 | 0.73 | 1.717 | 1.716 | 0.058 | 1.721 | 0.233 | 1.710 | 0.408 |
| 130.0 | 0.76 | 1.719 | 1.718 | 0.058 | 1.722 | 0.175 | 1.712 | 0.407 |
| 135.0 | 0.79 | 1.720 | 1.719 | 0.058 | 1.724 | 0.233 | 1.713 | 0.407 |
| 140.0 | 0.81 | 1.721 | 1.721 | 0.000 | 1.726 | 0.291 | 1.715 | 0.349 |
| 145.0 | 0.84 | 1.723 | 1.722 | 0.058 | 1.728 | 0.290 | 1.716 | 0.406 |
| 150.0 | 0.87 | 1.724 | 1.724 | 0.000 | 1.729 | 0.290 | 1.718 | 0.348 |
| 155.0 | 0.90 | 1.725 | 1.725 | 0.000 | 1.731 | 0.348 | 1.719 | 0.348 |
| 160.0 | 0.93 | 1.727 | 1.726 | 0.058 | 1.732 | 0.290 | 1.721 | 0.347 |
| $\boldsymbol{\epsilon_{\mathrm{AVE}}}$**(%)** | | | | **0.083** | | **0.334** | | **0.390** |
| $\boldsymbol{\epsilon_{\mathrm{MAX}}}$**(%)** | | | | **0.360** | | **1.321** | | **0.720** |

**Table 5b.** Key properties of the radial distribution function as resulting from molecular dynamics (MD) simulations and from three integral equation theory approaches: the updated version of the isomorph-based empirically modified hypernetted chain approximation (IEMHNC) introduced in the present letter, the variational modified hypernetted-chain approximation (VMHNC) discussed in *G. Faussurier, Phys. Rev. E* **69**, *066402 (2004)* and the empirically modified hypernetted-chain approximation (EMHNC) presented in *W. Daughton, M. S. Murillo and L. Thode, Phys. Rev. E* **61**, *2129 (2000).* The absolute relative deviation $\epsilon_{\mathrm{r}}$ between the theoretical and the simulation results is also reported together with its average and maximum values (the average deviation is denoted as $\epsilon_{\mathrm{AVE}}$ and the maximum deviation is denoted as $\epsilon_{\mathrm{MAX}}$). **Results for the position of the first non-zero minimum in the case of $\boldsymbol{\kappa = 1.0}$**. The MD results are adopted from *T. Ott and M. Bonitz, Contrib. Plasma Phys.* **55**, *243 (2015).* Here $x = r/d$, where $d$ is the Wigner-Seitz radius.

| $\Gamma$ | $\Gamma/\Gamma_m$ | $x_{\mathrm{min1}}^{\mathrm{MD}}$ | $x_{\mathrm{min1}}^{\mathrm{IEMHNC}}$ | $\epsilon_{\mathrm{IEMHNC}}(\%)$ | $x_{\mathrm{min1}}^{\mathrm{VMHNC}}$ | $\epsilon_{\mathrm{VMHNC}}(\%)$ | $x_{\mathrm{min1}}^{\mathrm{EMHNC}}$ | $\epsilon_{\mathrm{EMHNC}}(\%)$ |
|---|---|---|---|---|---|---|---|---|
| 10.0 | 0.05 | 1.660 | 1.679 | 1.145 | 1.635 | 1.506 | 1.675 | 0.904 |
| 15.0 | 0.07 | 1.648 | 1.645 | 0.182 | 1.624 | 1.456 | 1.662 | 0.850 |
| 20.0 | 0.09 | 1.648 | 1.643 | 0.303 | 1.627 | 1.274 | 1.656 | 0.485 |
| 25.0 | 0.11 | 1.650 | 1.649 | 0.061 | 1.632 | 1.091 | 1.655 | 0.303 |
| 30.0 | 0.14 | 1.655 | 1.655 | 0.000 | 1.638 | 1.027 | 1.656 | 0.060 |
| 35.0 | 0.16 | 1.659 | 1.661 | 0.121 | 1.644 | 0.904 | 1.657 | 0.121 |
| 40.0 | 0.18 | 1.662 | 1.665 | 0.181 | 1.650 | 0.722 | 1.660 | 0.120 |
| 45.0 | 0.20 | 1.666 | 1.669 | 0.180 | 1.655 | 0.660 | 1.662 | 0.240 |
| 50.0 | 0.23 | 1.669 | 1.672 | 0.180 | 1.660 | 0.539 | 1.665 | 0.240 |
| 55.0 | 0.25 | 1.673 | 1.675 | 0.120 | 1.664 | 0.538 | 1.668 | 0.299 |
| 60.0 | 0.27 | 1.676 | 1.677 | 0.060 | 1.668 | 0.477 | 1.670 | 0.358 |
| 65.0 | 0.30 | 1.679 | 1.679 | 0.000 | 1.672 | 0.417 | 1.673 | 0.357 |
| 70.0 | 0.32 | 1.681 | 1.681 | 0.000 | 1.676 | 0.297 | 1.675 | 0.357 |
| 75.0 | 0.34 | 1.684 | 1.683 | 0.059 | 1.679 | 0.297 | 1.678 | 0.356 |
| 80.0 | 0.36 | 1.687 | 1.685 | 0.119 | 1.682 | 0.296 | 1.680 | 0.415 |
| 85.0 | 0.39 | 1.689 | 1.687 | 0.118 | 1.685 | 0.237 | 1.683 | 0.355 |
| 90.0 | 0.41 | 1.691 | 1.689 | 0.118 | 1.688 | 0.177 | 1.685 | 0.355 |
| 95.0 | 0.43 | 1.693 | 1.691 | 0.118 | 1.691 | 0.118 | 1.687 | 0.354 |
| 100.0 | 0.45 | 1.695 | 1.693 | 0.118 | 1.694 | 0.059 | 1.689 | 0.354 |
| 105.0 | 0.48 | 1.697 | 1.695 | 0.118 | 1.696 | 0.059 | 1.691 | 0.354 |
| 110.0 | 0.50 | 1.699 | 1.697 | 0.118 | 1.698 | 0.059 | 1.693 | 0.353 |
| 115.0 | 0.52 | 1.701 | 1.699 | 0.118 | 1.701 | 0.000 | 1.695 | 0.353 |
| 120.0 | 0.54 | 1.702 | 1.701 | 0.059 | 1.703 | 0.059 | 1.697 | 0.294 |
| 125.0 | 0.57 | 1.704 | 1.702 | 0.117 | 1.705 | 0.059 | 1.699 | 0.293 |
| 130.0 | 0.59 | 1.706 | 1.704 | 0.117 | 1.707 | 0.059 | 1.700 | 0.352 |
| 135.0 | 0.61 | 1.707 | 1.706 | 0.059 | 1.709 | 0.117 | 1.702 | 0.293 |
| 140.0 | 0.64 | 1.709 | 1.707 | 0.117 | 1.710 | 0.059 | 1.704 | 0.293 |
| 145.0 | 0.66 | 1.710 | 1.709 | 0.058 | 1.712 | 0.117 | 1.705 | 0.292 |
| 150.0 | 0.68 | 1.712 | 1.710 | 0.117 | 1.714 | 0.117 | 1.707 | 0.292 |
| 155.0 | 0.70 | 1.713 | 1.712 | 0.058 | 1.715 | 0.117 | 1.708 | 0.292 |
| 160.0 | 0.73 | 1.715 | 1.713 | 0.117 | 1.717 | 0.117 | 1.710 | 0.292 |
| 165.0 | 0.75 | 1.715 | 1.714 | 0.058 | 1.718 | 0.175 | 1.711 | 0.233 |
| 170.0 | 0.77 | 1.717 | 1.716 | 0.058 | 1.720 | 0.175 | 1.713 | 0.233 |
| 175.0 | 0.79 | 1.718 | 1.717 | 0.058 | 1.721 | 0.175 | 1.714 | 0.233 |
| 180.0 | 0.82 | 1.719 | 1.718 | 0.058 | 1.723 | 0.233 | 1.715 | 0.233 |
| 185.0 | 0.84 | 1.720 | 1.719 | 0.058 | 1.724 | 0.233 | 1.717 | 0.174 |
| 190.0 | 0.86 | 1.721 | 1.720 | 0.058 | 1.725 | 0.232 | 1.718 | 0.174 |
| 195.0 | 0.89 | 1.722 | 1.722 | 0.000 | 1.727 | 0.290 | 1.719 | 0.174 |
| 200.0 | 0.91 | 1.723 | 1.723 | 0.000 | 1.728 | 0.290 | 1.720 | 0.174 |
| $\boldsymbol{\epsilon_{\mathrm{AVE}}}(\%)$ | | | | **0.121** | | **0.380** | | **0.314** |
| $\boldsymbol{\epsilon_{\mathrm{MAX}}}(\%)$ | | | | **1.145** | | **1.506** | | **0.904** |

**Table 5c.** Key properties of the radial distribution function as resulting from molecular dynamics (MD) simulations and from three integral equation theory approaches: the updated version of the isomorph-based empirically modified hypernetted chain approximation (IEMHNC) introduced in the present letter, the variational modified hypernetted-chain approximation (VMHNC) discussed in *G. Faussurier, Phys. Rev. E* **69**, *066402 (2004)* and the empirically modified hypernetted-chain approximation (EMHNC) presented in *W. Daughton, M. S. Murillo and L. Thode, Phys. Rev. E* **61**, *2129 (2000)*. The absolute relative deviation $\epsilon_{\mathrm{r}}$ between the theoretical and the simulation results is also reported together with its average and maximum values (the average deviation is denoted as $\epsilon_{\mathrm{AVE}}$ and the maximum deviation is denoted as $\epsilon_{\mathrm{MAX}}$). **Results for the position of the first non-zero minimum in the case of $\boldsymbol{\kappa = 2.0}$**. The MD results are adopted from *T. Ott and M. Bonitz, Contrib. Plasma Phys.* **55**, *243 (2015)*. Here $x = r/d$, where $d$ is the Wigner-Seitz radius.

| $\Gamma$ | $\Gamma/\Gamma_m$ | $x_{\mathrm{min1}}^{\mathrm{MD}}$ | $x_{\mathrm{min1}}^{\mathrm{IEMHNC}}$ | $\epsilon_{\mathrm{IEMHNC}}(\%)$ | $x_{\mathrm{min1}}^{\mathrm{VMHNC}}$ | $\epsilon_{\mathrm{VMHNC}}(\%)$ | $x_{\mathrm{min1}}^{\mathrm{EMHNC}}$ | $\epsilon_{\mathrm{EMHNC}}(\%)$ |
|---|---|---|---|---|---|---|---|---|
| 30.0 | 0.07 | 1.598 | 1.597 | 0.063 | 1.580 | 1.126 | 1.609 | 0.688 |
| 40.0 | 0.09 | 1.609 | 1.605 | 0.249 | 1.592 | 1.057 | 1.615 | 0.373 |
| 50.0 | 0.11 | 1.619 | 1.616 | 0.185 | 1.603 | 0.988 | 1.622 | 0.185 |
| 60.0 | 0.13 | 1.627 | 1.627 | 0.000 | 1.613 | 0.860 | 1.629 | 0.123 |
| 70.0 | 0.15 | 1.633 | 1.635 | 0.122 | 1.621 | 0.735 | 1.635 | 0.122 |
| 80.0 | 0.17 | 1.640 | 1.642 | 0.122 | 1.629 | 0.671 | 1.640 | 0.000 |
| 90.0 | 0.20 | 1.646 | 1.648 | 0.122 | 1.636 | 0.608 | 1.645 | 0.061 |
| 100.0 | 0.22 | 1.651 | 1.652 | 0.061 | 1.642 | 0.545 | 1.650 | 0.061 |
| 110.0 | 0.24 | 1.656 | 1.656 | 0.000 | 1.647 | 0.543 | 1.655 | 0.060 |
| 120.0 | 0.26 | 1.660 | 1.660 | 0.000 | 1.653 | 0.422 | 1.659 | 0.060 |
| 130.0 | 0.28 | 1.664 | 1.663 | 0.060 | 1.657 | 0.421 | 1.663 | 0.060 |
| 140.0 | 0.31 | 1.668 | 1.666 | 0.120 | 1.662 | 0.360 | 1.667 | 0.060 |
| 150.0 | 0.33 | 1.671 | 1.669 | 0.120 | 1.666 | 0.299 | 1.671 | 0.000 |
| 160.0 | 0.35 | 1.674 | 1.672 | 0.119 | 1.670 | 0.239 | 1.674 | 0.000 |
| 170.0 | 0.37 | 1.677 | 1.674 | 0.179 | 1.673 | 0.239 | 1.677 | 0.000 |
| 180.0 | 0.39 | 1.680 | 1.677 | 0.179 | 1.676 | 0.238 | 1.680 | 0.000 |
| 190.0 | 0.41 | 1.683 | 1.679 | 0.238 | 1.680 | 0.178 | 1.683 | 0.000 |
| 200.0 | 0.44 | 1.685 | 1.681 | 0.237 | 1.682 | 0.178 | 1.686 | 0.059 |
| 210.0 | 0.46 | 1.687 | 1.684 | 0.178 | 1.685 | 0.119 | 1.689 | 0.119 |
| 220.0 | 0.48 | 1.690 | 1.686 | 0.237 | 1.688 | 0.118 | 1.691 | 0.059 |
| 230.0 | 0.50 | 1.691 | 1.688 | 0.177 | 1.691 | 0.000 | 1.694 | 0.177 |
| 240.0 | 0.52 | 1.693 | 1.690 | 0.177 | 1.693 | 0.000 | 1.696 | 0.177 |
| 250.0 | 0.55 | 1.696 | 1.692 | 0.236 | 1.695 | 0.059 | 1.698 | 0.118 |
| 260.0 | 0.57 | 1.698 | 1.694 | 0.236 | 1.697 | 0.059 | 1.701 | 0.177 |
| 270.0 | 0.59 | 1.699 | 1.696 | 0.177 | 1.700 | 0.059 | 1.703 | 0.235 |
| 280.0 | 0.61 | 1.701 | 1.698 | 0.176 | 1.702 | 0.059 | 1.705 | 0.235 |
| 290.0 | 0.63 | 1.703 | 1.700 | 0.176 | 1.704 | 0.059 | 1.707 | 0.235 |
| 300.0 | 0.65 | 1.704 | 1.701 | 0.176 | 1.705 | 0.059 | 1.709 | 0.293 |
| 310.0 | 0.68 | 1.706 | 1.703 | 0.176 | 1.707 | 0.059 | 1.710 | 0.234 |
| 320.0 | 0.70 | 1.708 | 1.704 | 0.234 | 1.709 | 0.059 | 1.712 | 0.234 |
| 330.0 | 0.72 | 1.709 | 1.706 | 0.176 | 1.711 | 0.117 | 1.714 | 0.293 |
| 340.0 | 0.74 | 1.711 | 1.707 | 0.234 | 1.712 | 0.058 | 1.716 | 0.292 |
| 350.0 | 0.76 | 1.712 | 1.709 | 0.175 | 1.714 | 0.117 | 1.717 | 0.292 |
| 360.0 | 0.79 | 1.713 | 1.710 | 0.175 | 1.715 | 0.117 | 1.719 | 0.350 |
| 370.0 | 0.81 | 1.715 | 1.712 | 0.175 | 1.717 | 0.117 | 1.720 | 0.292 |
| 380.0 | 0.83 | 1.716 | 1.713 | 0.175 | 1.718 | 0.117 | 1.722 | 0.350 |
| 390.0 | 0.85 | 1.717 | 1.714 | 0.175 | 1.720 | 0.175 | 1.723 | 0.349 |
| 400.0 | 0.87 | 1.718 | 1.715 | 0.175 | 1.721 | 0.175 | 1.724 | 0.349 |
| $\boldsymbol{\epsilon_{\mathrm{AVE}}}(\%)$ | | | | **0.158** | | **0.300** | | **0.178** |
| $\boldsymbol{\epsilon_{\mathrm{MAX}}}(\%)$ | | | | **0.249** | | **1.126** | | **0.688** |

**Table 6a.** Key properties of the radial distribution function as resulting from molecular dynamics (MD) simulations and from three integral equation theory approaches: the updated version of the isomorph-based empirically modified hypernetted chain approximation (IEMHNC) introduced in the present letter, the variational modified hypernetted-chain approximation (VMHNC) discussed in *G. Faussurier, Phys. Rev. E* **69**, *066402 (2004)* and the empirically modified hypernetted-chain approximation (EMHNC) presented in *W. Daughton, M. S. Murillo and L. Thode, Phys. Rev. E* **61**, *2129 (2000)*. The absolute relative deviation $\epsilon_{\mathrm{r}}$ between the theoretical and the simulation results is also reported together with its average and maximum values (the average deviation is denoted as $\epsilon_{\mathrm{AVE}}$ and the maximum deviation is denoted as $\epsilon_{\mathrm{MAX}}$). **Results for the magnitude of the second maximum in the case of $\boldsymbol{\kappa = 0.0}$**. The MD results are adopted from *T. Ott and M. Bonitz, Contrib. Plasma Phys.* **55**, *243 (2015)*.

| $\Gamma$ | $\Gamma/\Gamma_m$ | $g_{\mathrm{max2}}^{\mathrm{MD}}$ | $g_{\mathrm{max2}}^{\mathrm{IEMHNC}}$ | $\epsilon_{\mathrm{IEMHNC}}(\%)$ | $g_{\mathrm{max2}}^{\mathrm{VMHNC}}$ | $\epsilon_{\mathrm{VMHNC}}(\%)$ | $g_{\mathrm{max2}}^{\mathrm{EMHNC}}$ | $\epsilon_{\mathrm{EMHNC}}(\%)$ |
|---|---|---|---|---|---|---|---|---|
| 15.0 | 0.09 | 1.228 | 1.227 | 0.081 | 1.228 | 0.000 | 1.200 | 2.280 |
| 20.0 | 0.12 | 1.307 | 1.307 | 0.000 | 1.312 | 0.383 | 1.277 | 2.295 |
| 25.0 | 0.15 | 1.378 | 1.378 | 0.000 | 1.387 | 0.653 | 1.348 | 2.177 |
| 30.0 | 0.17 | 1.443 | 1.442 | 0.069 | 1.457 | 0.970 | 1.414 | 2.010 |
| 35.0 | 0.20 | 1.504 | 1.502 | 0.133 | 1.521 | 1.130 | 1.475 | 1.928 |
| 40.0 | 0.23 | 1.560 | 1.557 | 0.192 | 1.581 | 1.346 | 1.533 | 1.731 |
| 45.0 | 0.26 | 1.614 | 1.610 | 0.248 | 1.637 | 1.425 | 1.587 | 1.673 |
| 50.0 | 0.29 | 1.664 | 1.661 | 0.180 | 1.691 | 1.623 | 1.639 | 1.502 |
| 55.0 | 0.32 | 1.712 | 1.709 | 0.175 | 1.741 | 1.694 | 1.688 | 1.402 |
| 60.0 | 0.35 | 1.757 | 1.755 | 0.114 | 1.790 | 1.878 | 1.735 | 1.252 |
| 65.0 | 0.38 | 1.803 | 1.799 | 0.222 | 1.837 | 1.886 | 1.781 | 1.220 |
| 70.0 | 0.41 | 1.845 | 1.842 | 0.163 | 1.881 | 1.951 | 1.824 | 1.138 |
| 75.0 | 0.44 | 1.885 | 1.884 | 0.053 | 1.925 | 2.122 | 1.867 | 0.955 |
| 80.0 | 0.47 | 1.926 | 1.924 | 0.104 | 1.966 | 2.077 | 1.908 | 0.935 |
| 85.0 | 0.49 | 1.964 | 1.963 | 0.051 | 2.007 | 2.189 | 1.948 | 0.815 |
| 90.0 | 0.52 | 2.001 | 2.001 | 0.000 | 2.046 | 2.249 | 1.987 | 0.700 |
| 95.0 | 0.55 | 2.037 | 2.037 | 0.000 | 2.084 | 2.307 | 2.025 | 0.589 |
| 100.0 | 0.58 | 2.072 | 2.073 | 0.048 | 2.122 | 2.413 | 2.063 | 0.434 |
| 105.0 | 0.61 | 2.107 | 2.108 | 0.047 | 2.158 | 2.421 | 2.099 | 0.380 |
| 110.0 | 0.64 | 2.140 | 2.143 | 0.140 | 2.193 | 2.477 | 2.134 | 0.280 |
| 115.0 | 0.67 | 2.174 | 2.176 | 0.092 | 2.228 | 2.484 | 2.169 | 0.230 |
| 120.0 | 0.70 | 2.206 | 2.209 | 0.136 | 2.262 | 2.539 | 2.204 | 0.091 |
| 125.0 | 0.73 | 2.237 | 2.240 | 0.134 | 2.295 | 2.593 | 2.237 | 0.000 |
| 130.0 | 0.76 | 2.270 | 2.271 | 0.044 | 2.327 | 2.511 | 2.270 | 0.000 |
| 135.0 | 0.79 | 2.298 | 2.302 | 0.174 | 2.359 | 2.654 | 2.303 | 0.218 |
| 140.0 | 0.81 | 2.329 | 2.331 | 0.086 | 2.390 | 2.619 | 2.334 | 0.215 |
| 145.0 | 0.84 | 2.358 | 2.360 | 0.085 | 2.421 | 2.672 | 2.366 | 0.339 |
| 150.0 | 0.87 | 2.386 | 2.388 | 0.084 | 2.451 | 2.724 | 2.397 | 0.461 |
| 155.0 | 0.90 | 2.413 | 2.416 | 0.124 | 2.481 | 2.818 | 2.427 | 0.580 |
| 160.0 | 0.93 | 2.442 | 2.442 | 0.000 | 2.510 | 2.785 | 2.457 | 0.614 |
| $\boldsymbol{\epsilon_{\mathrm{AVE}}}(\%)$ | | | | **0.099** | | **1.986** | | **0.948** |
| $\boldsymbol{\epsilon_{\mathrm{MAX}}}(\%)$ | | | | **0.248** | | **2.818** | | **2.295** |

**Table 6b.** Key properties of the radial distribution function as resulting from molecular dynamics (MD) simulations and from three integral equation theory approaches: the updated version of the isomorph-based empirically modified hypernetted chain approximation (IEMHNC) introduced in the present letter, the variational modified hypernetted-chain approximation (VMHNC) discussed in *G. Faussurier, Phys. Rev. E* **69**, *066402 (2004)* and the empirically modified hypernetted-chain approximation (EMHNC) presented in *W. Daughton, M. S. Murillo and L. Thode, Phys. Rev. E* **61**, *2129 (2000).* The absolute relative deviation $\epsilon_{\mathrm{r}}$ between the theoretical and the simulation results is also reported together with its average and maximum values (the average deviation is denoted as $\epsilon_{\mathrm{AVE}}$ and the maximum deviation is denoted as $\epsilon_{\mathrm{MAX}}$). **Results for the magnitude of the second maximum in the case of $\boldsymbol{\kappa = 1.0}$**. The MD results are adopted from *T. Ott and M. Bonitz, Contrib. Plasma Phys.* **55**, *243 (2015).*

| $\Gamma$ | $\Gamma/\Gamma_m$ | $g_{\mathrm{max2}}^{\mathrm{MD}}$ | $g_{\mathrm{max2}}^{\mathrm{IEMHNC}}$ | $\epsilon_{\mathrm{IEMHNC}}(\%)$ | $g_{\mathrm{max2}}^{\mathrm{VMHNC}}$ | $\epsilon_{\mathrm{VMHNC}}(\%)$ | $g_{\mathrm{max2}}^{\mathrm{EMHNC}}$ | $\epsilon_{\mathrm{EMHNC}}(\%)$ |
|---|---|---|---|---|---|---|---|---|
| 10.0 | 0.05 | 1.101 | 1.100 | 0.091 | 1.097 | 0.363 | 1.089 | 1.090 |
| 15.0 | 0.07 | 1.175 | 1.176 | 0.085 | 1.174 | 0.085 | 1.159 | 1.362 |
| 20.0 | 0.09 | 1.243 | 1.246 | 0.241 | 1.245 | 0.161 | 1.225 | 1.448 |
| 25.0 | 0.11 | 1.304 | 1.309 | 0.383 | 1.310 | 0.460 | 1.288 | 1.227 |
| 30.0 | 0.14 | 1.360 | 1.365 | 0.368 | 1.370 | 0.735 | 1.345 | 1.103 |
| 35.0 | 0.16 | 1.413 | 1.418 | 0.354 | 1.426 | 0.920 | 1.400 | 0.920 |
| 40.0 | 0.18 | 1.462 | 1.466 | 0.274 | 1.478 | 1.094 | 1.450 | 0.821 |
| 45.0 | 0.20 | 1.509 | 1.513 | 0.265 | 1.528 | 1.259 | 1.499 | 0.663 |
| 50.0 | 0.23 | 1.553 | 1.557 | 0.258 | 1.575 | 1.417 | 1.544 | 0.580 |
| 55.0 | 0.25 | 1.595 | 1.599 | 0.251 | 1.619 | 1.505 | 1.588 | 0.439 |
| 60.0 | 0.27 | 1.636 | 1.640 | 0.244 | 1.662 | 1.589 | 1.630 | 0.367 |
| 65.0 | 0.30 | 1.675 | 1.679 | 0.239 | 1.704 | 1.731 | 1.670 | 0.299 |
| 70.0 | 0.32 | 1.711 | 1.717 | 0.351 | 1.743 | 1.870 | 1.709 | 0.117 |
| 75.0 | 0.34 | 1.749 | 1.753 | 0.229 | 1.781 | 1.830 | 1.747 | 0.114 |
| 80.0 | 0.36 | 1.783 | 1.789 | 0.337 | 1.818 | 1.963 | 1.784 | 0.056 |
| 85.0 | 0.39 | 1.817 | 1.823 | 0.330 | 1.854 | 2.036 | 1.819 | 0.110 |
| 90.0 | 0.41 | 1.850 | 1.857 | 0.378 | 1.889 | 2.108 | 1.854 | 0.216 |
| 95.0 | 0.43 | 1.882 | 1.890 | 0.425 | 1.923 | 2.179 | 1.888 | 0.319 |
| 100.0 | 0.45 | 1.914 | 1.921 | 0.366 | 1.956 | 2.194 | 1.921 | 0.366 |
| 105.0 | 0.48 | 1.944 | 1.953 | 0.463 | 1.988 | 2.263 | 1.953 | 0.463 |
| 110.0 | 0.50 | 1.974 | 1.983 | 0.456 | 2.020 | 2.330 | 1.985 | 0.557 |
| 115.0 | 0.52 | 2.003 | 2.013 | 0.499 | 2.051 | 2.396 | 2.016 | 0.649 |
| 120.0 | 0.54 | 2.031 | 2.042 | 0.542 | 2.081 | 2.462 | 2.046 | 0.739 |
| 125.0 | 0.57 | 2.058 | 2.070 | 0.583 | 2.110 | 2.527 | 2.076 | 0.875 |
| 130.0 | 0.59 | 2.088 | 2.098 | 0.479 | 2.139 | 2.443 | 2.106 | 0.862 |
| 135.0 | 0.61 | 2.114 | 2.126 | 0.568 | 2.167 | 2.507 | 2.134 | 0.946 |
| 140.0 | 0.64 | 2.141 | 2.153 | 0.560 | 2.195 | 2.522 | 2.163 | 1.028 |
| 145.0 | 0.66 | 2.166 | 2.179 | 0.600 | 2.222 | 2.585 | 2.191 | 1.154 |
| 150.0 | 0.68 | 2.191 | 2.205 | 0.639 | 2.249 | 2.647 | 2.218 | 1.232 |
| 155.0 | 0.70 | 2.217 | 2.230 | 0.586 | 2.276 | 2.661 | 2.245 | 1.263 |
| 160.0 | 0.73 | 2.242 | 2.255 | 0.580 | 2.302 | 2.676 | 2.272 | 1.338 |
| 165.0 | 0.75 | 2.266 | 2.280 | 0.618 | 2.327 | 2.692 | 2.299 | 1.456 |
| 170.0 | 0.77 | 2.289 | 2.304 | 0.655 | 2.352 | 2.752 | 2.325 | 1.573 |
| 175.0 | 0.79 | 2.314 | 2.327 | 0.562 | 2.377 | 2.723 | 2.350 | 1.556 |
| 180.0 | 0.82 | 2.337 | 2.350 | 0.556 | 2.402 | 2.781 | 2.376 | 1.669 |
| 185.0 | 0.84 | 2.359 | 2.373 | 0.593 | 2.426 | 2.840 | 2.401 | 1.780 |
| 190.0 | 0.86 | 2.383 | 2.395 | 0.504 | 2.450 | 2.812 | 2.425 | 1.762 |
| 195.0 | 0.89 | 2.404 | 2.417 | 0.541 | 2.473 | 2.870 | 2.450 | 1.913 |
| 200.0 | 0.91 | 2.427 | 2.439 | 0.494 | 2.496 | 2.843 | 2.474 | 1.937 |
| $\boldsymbol{\epsilon_{\mathrm{AVE}}}(\%)$ | | | | **0.424** | | **1.996** | | **0.932** |
| $\boldsymbol{\epsilon_{\mathrm{MAX}}}(\%)$ | | | | **0.655** | | **2.870** | | **1.937** |

**Table 6c.** Key properties of the radial distribution function as resulting from molecular dynamics (MD) simulations and from three integral equation theory approaches: the updated version of the isomorph-based empirically modified hypernetted chain approximation (IEMHNC) introduced in the present letter, the variational modified hypernetted-chain approximation (VMHNC) discussed in *G. Faussurier, Phys. Rev. E* **69**, *066402 (2004)* and the empirically modified hypernetted-chain approximation (EMHNC) presented in *W. Daughton, M. S. Murillo and L. Thode, Phys. Rev. E* **61**, *2129 (2000)*. The absolute relative deviation $\epsilon_{\mathrm{r}}$ between the theoretical and the simulation results is also reported together with its average and maximum values (the average deviation is denoted as $\epsilon_{\mathrm{AVE}}$ and the maximum deviation is denoted as $\epsilon_{\mathrm{MAX}}$). **Results for the magnitude of the second maximum in the case of $\boldsymbol{\kappa = 2.0}$**. The MD results are adopted from *T. Ott and M. Bonitz, Contrib. Plasma Phys.* **55**, *243 (2015)*.

| $\Gamma$ | $\Gamma/\Gamma_m$ | $g_{\mathrm{max2}}^{\mathrm{MD}}$ | $g_{\mathrm{max2}}^{\mathrm{IEMHNC}}$ | $\epsilon_{\mathrm{IEMHNC}}(\%)$ | $g_{\mathrm{max2}}^{\mathrm{VMHNC}}$ | $\epsilon_{\mathrm{VMHNC}}(\%)$ | $g_{\mathrm{max2}}^{\mathrm{EMHNC}}$ | $\epsilon_{\mathrm{EMHNC}}(\%)$ |
|---|---|---|---|---|---|---|---|---|
| 30.0 | 0.07 | 1.202 | 1.202 | 0.000 | 1.206 | 0.333 | 1.201 | 0.083 |
| 40.0 | 0.09 | 1.270 | 1.274 | 0.315 | 1.277 | 0.551 | 1.273 | 0.236 |
| 50.0 | 0.11 | 1.331 | 1.337 | 0.451 | 1.342 | 0.826 | 1.337 | 0.451 |
| 60.0 | 0.13 | 1.388 | 1.393 | 0.360 | 1.402 | 1.009 | 1.397 | 0.648 |
| 70.0 | 0.15 | 1.440 | 1.446 | 0.417 | 1.458 | 1.250 | 1.453 | 0.903 |
| 80.0 | 0.17 | 1.490 | 1.495 | 0.336 | 1.510 | 1.342 | 1.505 | 1.007 |
| 90.0 | 0.20 | 1.536 | 1.542 | 0.391 | 1.560 | 1.563 | 1.554 | 1.172 |
| 100.0 | 0.22 | 1.582 | 1.586 | 0.253 | 1.607 | 1.580 | 1.601 | 1.201 |
| 110.0 | 0.24 | 1.624 | 1.629 | 0.308 | 1.652 | 1.724 | 1.646 | 1.355 |
| 120.0 | 0.26 | 1.664 | 1.670 | 0.361 | 1.695 | 1.863 | 1.689 | 1.502 |
| 130.0 | 0.28 | 1.702 | 1.710 | 0.470 | 1.736 | 1.998 | 1.731 | 1.704 |
| 140.0 | 0.31 | 1.741 | 1.748 | 0.402 | 1.776 | 2.010 | 1.771 | 1.723 |
| 150.0 | 0.33 | 1.777 | 1.785 | 0.450 | 1.815 | 2.138 | 1.810 | 1.857 |
| 160.0 | 0.35 | 1.812 | 1.821 | 0.497 | 1.852 | 2.208 | 1.848 | 1.987 |
| 170.0 | 0.37 | 1.847 | 1.856 | 0.487 | 1.888 | 2.220 | 1.885 | 2.057 |
| 180.0 | 0.39 | 1.879 | 1.890 | 0.585 | 1.923 | 2.342 | 1.921 | 2.235 |
| 190.0 | 0.41 | 1.912 | 1.923 | 0.575 | 1.958 | 2.406 | 1.957 | 2.354 |
| 200.0 | 0.44 | 1.944 | 1.955 | 0.566 | 1.991 | 2.418 | 1.991 | 2.418 |
| 210.0 | 0.46 | 1.974 | 1.987 | 0.659 | 2.024 | 2.533 | 2.025 | 2.584 |
| 220.0 | 0.48 | 2.004 | 2.017 | 0.649 | 2.055 | 2.545 | 2.057 | 2.645 |
| 230.0 | 0.50 | 2.034 | 2.047 | 0.639 | 2.087 | 2.606 | 2.090 | 2.753 |
| 240.0 | 0.52 | 2.062 | 2.077 | 0.727 | 2.117 | 2.667 | 2.121 | 2.861 |
| 250.0 | 0.55 | 2.091 | 2.106 | 0.717 | 2.147 | 2.678 | 2.152 | 2.917 |
| 260.0 | 0.57 | 2.119 | 2.134 | 0.708 | 2.176 | 2.690 | 2.183 | 3.020 |
| 270.0 | 0.59 | 2.145 | 2.161 | 0.746 | 2.205 | 2.797 | 2.213 | 3.170 |
| 280.0 | 0.61 | 2.173 | 2.189 | 0.736 | 2.233 | 2.761 | 2.243 | 3.221 |
| 290.0 | 0.63 | 2.198 | 2.215 | 0.773 | 2.261 | 2.866 | 2.272 | 3.367 |
| 300.0 | 0.65 | 2.225 | 2.241 | 0.719 | 2.288 | 2.831 | 2.300 | 3.371 |
| 310.0 | 0.68 | 2.250 | 2.267 | 0.756 | 2.315 | 2.889 | 2.328 | 3.467 |
| 320.0 | 0.70 | 2.274 | 2.292 | 0.792 | 2.341 | 2.946 | 2.356 | 3.606 |
| 330.0 | 0.72 | 2.299 | 2.317 | 0.783 | 2.367 | 2.958 | 2.383 | 3.654 |
| 340.0 | 0.74 | 2.324 | 2.342 | 0.775 | 2.393 | 2.969 | 2.410 | 3.701 |
| 350.0 | 0.76 | 2.347 | 2.365 | 0.767 | 2.418 | 3.025 | 2.436 | 3.792 |
| 360.0 | 0.79 | 2.371 | 2.389 | 0.759 | 2.443 | 3.037 | 2.463 | 3.880 |
| 370.0 | 0.81 | 2.394 | 2.412 | 0.752 | 2.468 | 3.091 | 2.488 | 3.926 |
| 380.0 | 0.83 | 2.417 | 2.435 | 0.745 | 2.492 | 3.103 | 2.514 | 4.013 |
| 390.0 | 0.85 | 2.438 | 2.457 | 0.779 | 2.516 | 3.199 | 2.539 | 4.143 |
| 400.0 | 0.87 | 2.462 | 2.479 | 0.690 | 2.539 | 3.128 | 2.563 | 4.102 |
| $\boldsymbol{\epsilon_{\mathrm{AVE}}}(\%)$ | | | | **0.576** | | **2.292** | | **2.450** |
| $\boldsymbol{\epsilon_{\mathrm{MAX}}}(\%)$ | | | | **0.792** | | **3.199** | | **4.143** |

**Table 7a.** Key properties of the radial distribution function as resulting from molecular dynamics (MD) simulations and from three integral equation theory approaches: the updated version of the isomorph-based empirically modified hypernetted chain approximation (IEMHNC) introduced in the present letter, the variational modified hypernetted-chain approximation (VMHNC) discussed in *G. Faussurier, Phys. Rev. E* **69**, *066402 (2004)* and the empirically modified hypernetted-chain approximation (EMHNC) presented in *W. Daughton, M. S. Murillo and L. Thode, Phys. Rev. E* **61**, *2129 (2000)*. The absolute relative deviation $\epsilon_{\mathrm{r}}$ between the theoretical and the simulation results is also reported together with its average and maximum values (the average deviation is denoted as $\epsilon_{\mathrm{AVE}}$ and the maximum deviation is denoted as $\epsilon_{\mathrm{MAX}}$). **Results for the position of the second maximum in the case of $\boldsymbol{\kappa = 0.0}$**. The MD results are adopted from *T. Ott and M. Bonitz, Contrib. Plasma Phys.* **55**, *243 (2015)*. Here $x = r/d$, where $d$ is the Wigner-Seitz radius.

| $\Gamma$ | $\Gamma/\Gamma_m$ | $x_{\mathrm{max2}}^{\mathrm{MD}}$ | $x_{\mathrm{max2}}^{\mathrm{IEMHNC}}$ | $\epsilon_{\mathrm{IEMHNC}}(\%)$ | $x_{\mathrm{max2}}^{\mathrm{VMHNC}}$ | $\epsilon_{\mathrm{VMHNC}}(\%)$ | $x_{\mathrm{max2}}^{\mathrm{EMHNC}}$ | $\epsilon_{\mathrm{EMHNC}}(\%)$ |
|---|---|---|---|---|---|---|---|---|
| 15.0 | 0.09 | 1.666 | 1.660 | 0.360 | 1.644 | 1.321 | 1.678 | 0.720 |
| 20.0 | 0.12 | 1.665 | 1.663 | 0.120 | 1.647 | 1.081 | 1.672 | 0.420 |
| 25.0 | 0.15 | 1.668 | 1.669 | 0.060 | 1.652 | 0.959 | 1.670 | 0.120 |
| 30.0 | 0.17 | 1.671 | 1.674 | 0.180 | 1.658 | 0.778 | 1.670 | 0.060 |
| 35.0 | 0.20 | 1.674 | 1.678 | 0.239 | 1.664 | 0.597 | 1.671 | 0.179 |
| 40.0 | 0.23 | 1.678 | 1.680 | 0.119 | 1.669 | 0.536 | 1.673 | 0.298 |
| 45.0 | 0.26 | 1.681 | 1.683 | 0.119 | 1.674 | 0.416 | 1.676 | 0.297 |
| 50.0 | 0.29 | 1.685 | 1.685 | 0.000 | 1.678 | 0.415 | 1.678 | 0.415 |
| 55.0 | 0.32 | 1.688 | 1.688 | 0.000 | 1.683 | 0.296 | 1.681 | 0.415 |
| 60.0 | 0.35 | 1.690 | 1.690 | 0.000 | 1.687 | 0.178 | 1.683 | 0.414 |
| 65.0 | 0.38 | 1.693 | 1.692 | 0.059 | 1.690 | 0.177 | 1.686 | 0.413 |
| 70.0 | 0.41 | 1.696 | 1.694 | 0.118 | 1.694 | 0.118 | 1.688 | 0.472 |
| 75.0 | 0.44 | 1.698 | 1.697 | 0.059 | 1.697 | 0.059 | 1.690 | 0.471 |
| 80.0 | 0.47 | 1.701 | 1.699 | 0.118 | 1.700 | 0.059 | 1.693 | 0.470 |
| 85.0 | 0.49 | 1.703 | 1.701 | 0.117 | 1.703 | 0.000 | 1.695 | 0.470 |
| 90.0 | 0.52 | 1.705 | 1.703 | 0.117 | 1.705 | 0.000 | 1.697 | 0.469 |
| 95.0 | 0.55 | 1.707 | 1.705 | 0.117 | 1.708 | 0.059 | 1.699 | 0.469 |
| 100.0 | 0.58 | 1.709 | 1.707 | 0.117 | 1.710 | 0.059 | 1.701 | 0.468 |
| 105.0 | 0.61 | 1.710 | 1.709 | 0.058 | 1.713 | 0.175 | 1.703 | 0.409 |
| 110.0 | 0.64 | 1.712 | 1.711 | 0.058 | 1.715 | 0.175 | 1.705 | 0.409 |
| 115.0 | 0.67 | 1.714 | 1.713 | 0.058 | 1.717 | 0.175 | 1.707 | 0.408 |
| 120.0 | 0.70 | 1.715 | 1.715 | 0.000 | 1.719 | 0.233 | 1.708 | 0.408 |
| 125.0 | 0.73 | 1.717 | 1.716 | 0.058 | 1.721 | 0.233 | 1.710 | 0.408 |
| 130.0 | 0.76 | 1.719 | 1.718 | 0.058 | 1.722 | 0.175 | 1.712 | 0.407 |
| 135.0 | 0.79 | 1.720 | 1.719 | 0.058 | 1.724 | 0.233 | 1.713 | 0.407 |
| 140.0 | 0.81 | 1.721 | 1.721 | 0.000 | 1.726 | 0.291 | 1.715 | 0.349 |
| 145.0 | 0.84 | 1.723 | 1.722 | 0.058 | 1.728 | 0.290 | 1.716 | 0.406 |
| 150.0 | 0.87 | 1.724 | 1.724 | 0.000 | 1.729 | 0.290 | 1.718 | 0.348 |
| 155.0 | 0.90 | 1.725 | 1.725 | 0.000 | 1.731 | 0.348 | 1.719 | 0.348 |
| 160.0 | 0.93 | 1.727 | 1.726 | 0.058 | 1.732 | 0.290 | 1.721 | 0.347 |
| $\boldsymbol{\epsilon_{\mathrm{AVE}}}(\%)$ | | | | **0.083** | | **0.334** | | **0.390** |
| $\boldsymbol{\epsilon_{\mathrm{MAX}}}(\%)$ | | | | **0.360** | | **1.321** | | **0.720** |

**Table 7b.** Key properties of the radial distribution function as resulting from molecular dynamics (MD) simulations and from three integral equation theory approaches: the updated version of the isomorph-based empirically modified hypernetted chain approximation (IEMHNC) introduced in the present letter, the variational modified hypernetted-chain approximation (VMHNC) discussed in *G. Faussurier, Phys. Rev. E* **69**, *066402 (2004)* and the empirically modified hypernetted-chain approximation (EMHNC) presented in *W. Daughton, M. S. Murillo and L. Thode, Phys. Rev. E* **61**, *2129 (2000)*. The absolute relative deviation $\epsilon_{\mathrm{r}}$ between the theoretical and the simulation results is also reported together with its average and maximum values (the average deviation is denoted as $\epsilon_{\mathrm{AVE}}$ and the maximum deviation is denoted as $\epsilon_{\mathrm{MAX}}$). **Results for the position of the second maximum in the case of $\boldsymbol{\kappa = 1.0}$.** The MD results are adopted from *T. Ott and M. Bonitz, Contrib. Plasma Phys.* **55**, *243 (2015)*. Here $x = r/d$, where $d$ is the Wigner-Seitz radius.

| $\Gamma$ | $\Gamma/\Gamma_m$ | $x_{\mathrm{max2}}^{\mathrm{MD}}$ | $x_{\mathrm{max2}}^{\mathrm{IEMHNC}}$ | $\epsilon_{\mathrm{IEMHNC}}(\%)$ | $x_{\mathrm{max2}}^{\mathrm{VMHNC}}$ | $\epsilon_{\mathrm{VMHNC}}(\%)$ | $x_{\mathrm{max2}}^{\mathrm{EMHNC}}$ | $\epsilon_{\mathrm{EMHNC}}(\%)$ |
|---|---|---|---|---|---|---|---|---|
| 10.0 | 0.05 | 1.660 | 1.679 | 1.145 | 1.635 | 1.506 | 1.675 | 0.904 |
| 15.0 | 0.07 | 1.648 | 1.645 | 0.182 | 1.624 | 1.456 | 1.662 | 0.850 |
| 20.0 | 0.09 | 1.648 | 1.643 | 0.303 | 1.627 | 1.274 | 1.656 | 0.485 |
| 25.0 | 0.11 | 1.650 | 1.649 | 0.061 | 1.632 | 1.091 | 1.655 | 0.303 |
| 30.0 | 0.14 | 1.655 | 1.655 | 0.000 | 1.638 | 1.027 | 1.656 | 0.060 |
| 35.0 | 0.16 | 1.659 | 1.661 | 0.121 | 1.644 | 0.904 | 1.657 | 0.121 |
| 40.0 | 0.18 | 1.662 | 1.665 | 0.181 | 1.650 | 0.722 | 1.660 | 0.120 |
| 45.0 | 0.20 | 1.666 | 1.669 | 0.180 | 1.655 | 0.660 | 1.662 | 0.240 |
| 50.0 | 0.23 | 1.669 | 1.672 | 0.180 | 1.660 | 0.539 | 1.665 | 0.240 |
| 55.0 | 0.25 | 1.673 | 1.675 | 0.120 | 1.664 | 0.538 | 1.668 | 0.299 |
| 60.0 | 0.27 | 1.676 | 1.677 | 0.060 | 1.668 | 0.477 | 1.670 | 0.358 |
| 65.0 | 0.30 | 1.679 | 1.679 | 0.000 | 1.672 | 0.417 | 1.673 | 0.357 |
| 70.0 | 0.32 | 1.681 | 1.681 | 0.000 | 1.676 | 0.297 | 1.675 | 0.357 |
| 75.0 | 0.34 | 1.684 | 1.683 | 0.059 | 1.679 | 0.297 | 1.678 | 0.356 |
| 80.0 | 0.36 | 1.687 | 1.685 | 0.119 | 1.682 | 0.296 | 1.680 | 0.415 |
| 85.0 | 0.39 | 1.689 | 1.687 | 0.118 | 1.685 | 0.237 | 1.683 | 0.355 |
| 90.0 | 0.41 | 1.691 | 1.689 | 0.118 | 1.688 | 0.177 | 1.685 | 0.355 |
| 95.0 | 0.43 | 1.693 | 1.691 | 0.118 | 1.691 | 0.118 | 1.687 | 0.354 |
| 100.0 | 0.45 | 1.695 | 1.693 | 0.118 | 1.694 | 0.059 | 1.689 | 0.354 |
| 105.0 | 0.48 | 1.697 | 1.695 | 0.118 | 1.696 | 0.059 | 1.691 | 0.354 |
| 110.0 | 0.50 | 1.699 | 1.697 | 0.118 | 1.698 | 0.059 | 1.693 | 0.353 |
| 115.0 | 0.52 | 1.701 | 1.699 | 0.118 | 1.701 | 0.000 | 1.695 | 0.353 |
| 120.0 | 0.54 | 1.702 | 1.701 | 0.059 | 1.703 | 0.059 | 1.697 | 0.294 |
| 125.0 | 0.57 | 1.704 | 1.702 | 0.117 | 1.705 | 0.059 | 1.699 | 0.293 |
| 130.0 | 0.59 | 1.706 | 1.704 | 0.117 | 1.707 | 0.059 | 1.700 | 0.352 |
| 135.0 | 0.61 | 1.707 | 1.706 | 0.059 | 1.709 | 0.117 | 1.702 | 0.293 |
| 140.0 | 0.64 | 1.709 | 1.707 | 0.117 | 1.710 | 0.059 | 1.704 | 0.293 |
| 145.0 | 0.66 | 1.710 | 1.709 | 0.058 | 1.712 | 0.117 | 1.705 | 0.292 |
| 150.0 | 0.68 | 1.712 | 1.710 | 0.117 | 1.714 | 0.117 | 1.707 | 0.292 |
| 155.0 | 0.70 | 1.713 | 1.712 | 0.058 | 1.715 | 0.117 | 1.708 | 0.292 |
| 160.0 | 0.73 | 1.715 | 1.713 | 0.117 | 1.717 | 0.117 | 1.710 | 0.292 |
| 165.0 | 0.75 | 1.715 | 1.714 | 0.058 | 1.718 | 0.175 | 1.711 | 0.233 |
| 170.0 | 0.77 | 1.717 | 1.716 | 0.058 | 1.720 | 0.175 | 1.713 | 0.233 |
| 175.0 | 0.79 | 1.718 | 1.717 | 0.058 | 1.721 | 0.175 | 1.714 | 0.233 |
| 180.0 | 0.82 | 1.719 | 1.718 | 0.058 | 1.723 | 0.233 | 1.715 | 0.233 |
| 185.0 | 0.84 | 1.720 | 1.719 | 0.058 | 1.724 | 0.233 | 1.717 | 0.174 |
| 190.0 | 0.86 | 1.721 | 1.720 | 0.058 | 1.725 | 0.232 | 1.718 | 0.174 |
| 195.0 | 0.89 | 1.722 | 1.722 | 0.000 | 1.727 | 0.290 | 1.719 | 0.174 |
| 200.0 | 0.91 | 1.723 | 1.723 | 0.000 | 1.728 | 0.290 | 1.720 | 0.174 |
| $\boldsymbol{\epsilon_{\mathrm{AVE}}}(\%)$ | | | | **0.121** | | **0.380** | | **0.314** |
| $\boldsymbol{\epsilon_{\mathrm{MAX}}}(\%)$ | | | | **1.145** | | **1.506** | | **0.904** |

**Table 7c.** Key properties of the radial distribution function as resulting from molecular dynamics (MD) simulations and from three integral equation theory approaches: the updated version of the isomorph-based empirically modified hypernetted chain approximation (IEMHNC) introduced in the present letter, the variational modified hypernetted-chain approximation (VMHNC) discussed in *G. Faussurier, Phys. Rev. E* **69**, *066402 (2004)* and the empirically modified hypernetted-chain approximation (EMHNC) presented in *W. Daughton, M. S. Murillo and L. Thode, Phys. Rev. E* **61**, *2129 (2000)*. The absolute relative deviation $\epsilon_{\mathrm{r}}$ between the theoretical and the simulation results is also reported together with its average and maximum values (the average deviation is denoted as $\epsilon_{\mathrm{AVE}}$ and the maximum deviation is denoted as $\epsilon_{\mathrm{MAX}}$). **Results for the position of the second maximum in the case of $\boldsymbol{\kappa = 2.0}$.** The MD results are adopted from *T. Ott and M. Bonitz, Contrib. Plasma Phys.* **55**, *243 (2015)*. Here $x = r/d$, where $d$ is the Wigner-Seitz radius.

| $\Gamma$ | $\Gamma/\Gamma_m$ | $x^{\mathrm{MD}}_{\mathrm{max2}}$ | $x^{\mathrm{IEMHNC}}_{\mathrm{max2}}$ | $\epsilon_{\mathrm{IEMHNC}}(\%)$ | $x^{\mathrm{VMHNC}}_{\mathrm{max2}}$ | $\epsilon_{\mathrm{VMHNC}}(\%)$ | $x^{\mathrm{EMHNC}}_{\mathrm{max2}}$ | $\epsilon_{\mathrm{EMHNC}}(\%)$ |
|---|---|---|---|---|---|---|---|---|
| 30.0 | 0.07 | 1.598 | 1.597 | 0.063 | 1.580 | 1.126 | 1.609 | 0.688 |
| 40.0 | 0.09 | 1.609 | 1.605 | 0.249 | 1.592 | 1.057 | 1.615 | 0.373 |
| 50.0 | 0.11 | 1.619 | 1.616 | 0.185 | 1.603 | 0.988 | 1.622 | 0.185 |
| 60.0 | 0.13 | 1.627 | 1.627 | 0.000 | 1.613 | 0.860 | 1.629 | 0.123 |
| 70.0 | 0.15 | 1.633 | 1.635 | 0.122 | 1.621 | 0.735 | 1.635 | 0.122 |
| 80.0 | 0.17 | 1.640 | 1.642 | 0.122 | 1.629 | 0.671 | 1.640 | 0.000 |
| 90.0 | 0.20 | 1.646 | 1.648 | 0.122 | 1.636 | 0.608 | 1.645 | 0.061 |
| 100.0 | 0.22 | 1.651 | 1.652 | 0.061 | 1.642 | 0.545 | 1.650 | 0.061 |
| 110.0 | 0.24 | 1.656 | 1.656 | 0.000 | 1.647 | 0.543 | 1.655 | 0.060 |
| 120.0 | 0.26 | 1.660 | 1.660 | 0.000 | 1.653 | 0.422 | 1.659 | 0.060 |
| 130.0 | 0.28 | 1.664 | 1.663 | 0.060 | 1.657 | 0.421 | 1.663 | 0.060 |
| 140.0 | 0.31 | 1.668 | 1.666 | 0.120 | 1.662 | 0.360 | 1.667 | 0.060 |
| 150.0 | 0.33 | 1.671 | 1.669 | 0.120 | 1.666 | 0.299 | 1.671 | 0.000 |
| 160.0 | 0.35 | 1.674 | 1.672 | 0.119 | 1.670 | 0.239 | 1.674 | 0.000 |
| 170.0 | 0.37 | 1.677 | 1.674 | 0.179 | 1.673 | 0.239 | 1.677 | 0.000 |
| 180.0 | 0.39 | 1.680 | 1.677 | 0.179 | 1.676 | 0.238 | 1.680 | 0.000 |
| 190.0 | 0.41 | 1.683 | 1.679 | 0.238 | 1.680 | 0.178 | 1.683 | 0.000 |
| 200.0 | 0.44 | 1.685 | 1.681 | 0.237 | 1.682 | 0.178 | 1.686 | 0.059 |
| 210.0 | 0.46 | 1.687 | 1.684 | 0.178 | 1.685 | 0.119 | 1.689 | 0.119 |
| 220.0 | 0.48 | 1.690 | 1.686 | 0.237 | 1.688 | 0.118 | 1.691 | 0.059 |
| 230.0 | 0.50 | 1.691 | 1.688 | 0.177 | 1.691 | 0.000 | 1.694 | 0.177 |
| 240.0 | 0.52 | 1.693 | 1.690 | 0.177 | 1.693 | 0.000 | 1.696 | 0.177 |
| 250.0 | 0.55 | 1.696 | 1.692 | 0.236 | 1.695 | 0.059 | 1.698 | 0.118 |
| 260.0 | 0.57 | 1.698 | 1.694 | 0.236 | 1.697 | 0.059 | 1.701 | 0.177 |
| 270.0 | 0.59 | 1.699 | 1.696 | 0.177 | 1.700 | 0.059 | 1.703 | 0.235 |
| 280.0 | 0.61 | 1.701 | 1.698 | 0.176 | 1.702 | 0.059 | 1.705 | 0.235 |
| 290.0 | 0.63 | 1.703 | 1.700 | 0.176 | 1.704 | 0.059 | 1.707 | 0.235 |
| 300.0 | 0.65 | 1.704 | 1.701 | 0.176 | 1.705 | 0.059 | 1.709 | 0.293 |
| 310.0 | 0.68 | 1.706 | 1.703 | 0.176 | 1.707 | 0.059 | 1.710 | 0.234 |
| 320.0 | 0.70 | 1.708 | 1.704 | 0.234 | 1.709 | 0.059 | 1.712 | 0.234 |
| 330.0 | 0.72 | 1.709 | 1.706 | 0.176 | 1.711 | 0.117 | 1.714 | 0.293 |
| 340.0 | 0.74 | 1.711 | 1.707 | 0.234 | 1.712 | 0.058 | 1.716 | 0.292 |
| 350.0 | 0.76 | 1.712 | 1.709 | 0.175 | 1.714 | 0.117 | 1.717 | 0.292 |
| 360.0 | 0.79 | 1.713 | 1.710 | 0.175 | 1.715 | 0.117 | 1.719 | 0.350 |
| 370.0 | 0.81 | 1.715 | 1.712 | 0.175 | 1.717 | 0.117 | 1.720 | 0.292 |
| 380.0 | 0.83 | 1.716 | 1.713 | 0.175 | 1.718 | 0.117 | 1.722 | 0.350 |
| 390.0 | 0.85 | 1.717 | 1.714 | 0.175 | 1.720 | 0.175 | 1.723 | 0.349 |
| 400.0 | 0.87 | 1.718 | 1.715 | 0.175 | 1.721 | 0.175 | 1.724 | 0.349 |
| $\boldsymbol{\epsilon_{\mathrm{AVE}}}(\%)$ | | | | **0.158** | | **0.300** | | **0.178** |
| $\boldsymbol{\epsilon_{\mathrm{MAX}}}(\%)$ | | | | **0.249** | | **1.126** | | **0.688** |

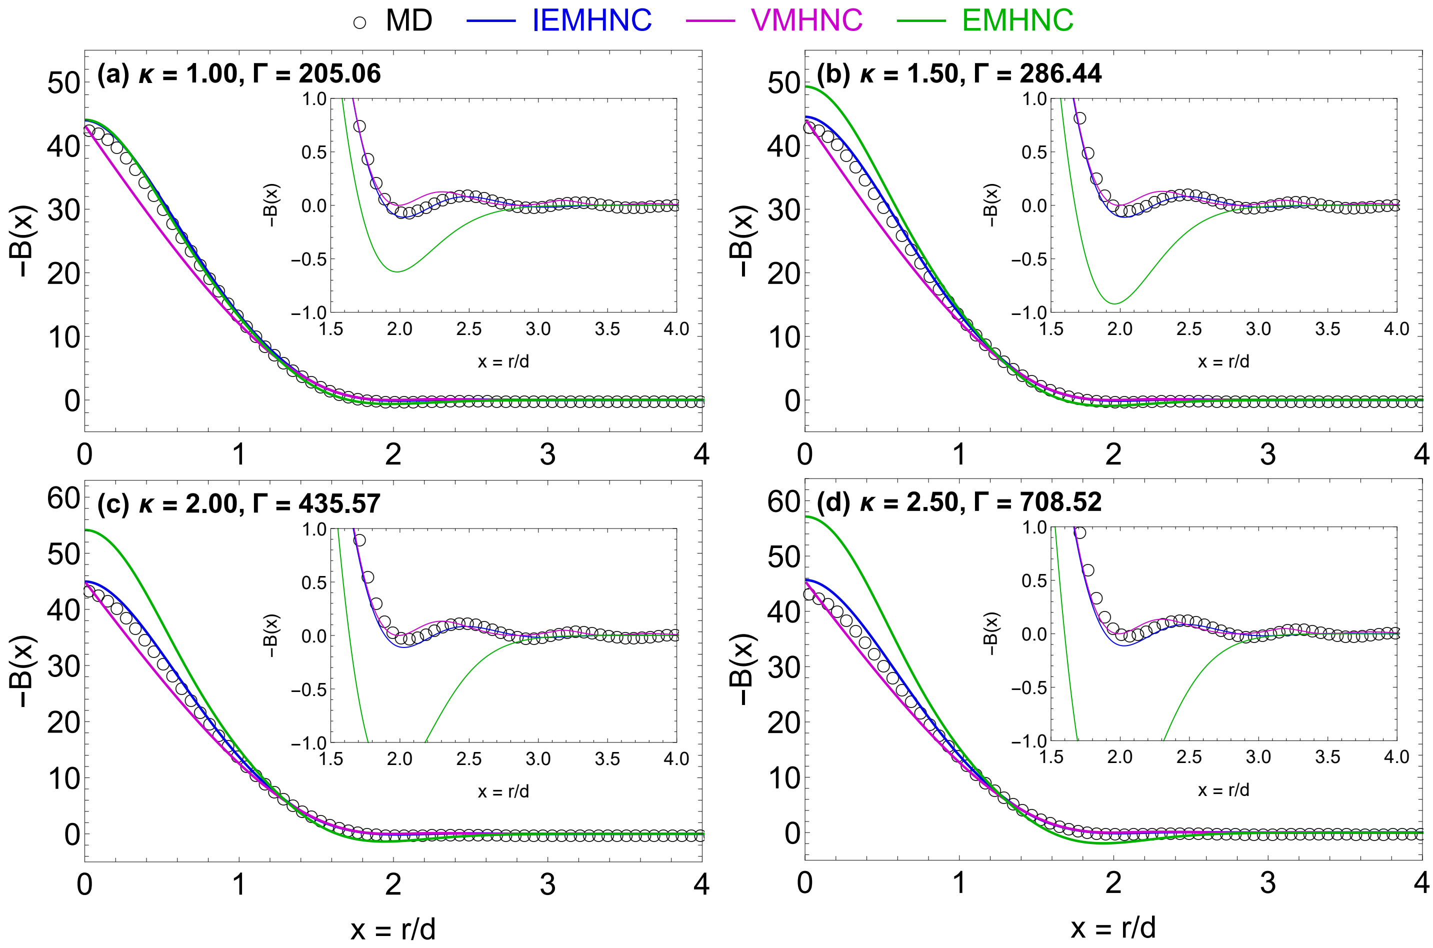


**Figure 1.** Bridge functions resulting from molecular dynamics (MD) simulations and from three integral equation theory approaches: the updated version of the isomorph-based empirically modified hypernetted chain approximation (IEMHNC) introduced in the present letter, the variational modified hypernetted-chain approximation (VMHNC) discussed in *G. Faussurier, Phys. Rev. E* **69**, *066402 (2004)* and the empirically modified hypernetted-chain approximation (EMHNC) presented in *W. Daughton, M. S. Murillo and L. Thode, Phys. Rev. E* **61**, *2129 (2000)*. The MD results are adopted from *F. Lucco Castello, P. Tolias and J. C. Dyre, J. Chem. Phys.* **154**, *034501 (2021)*. **Results for four YOCP state points that belong to the isomorphic line with reduced excess entropy $s_{\text{ex}} = -3.880$.**

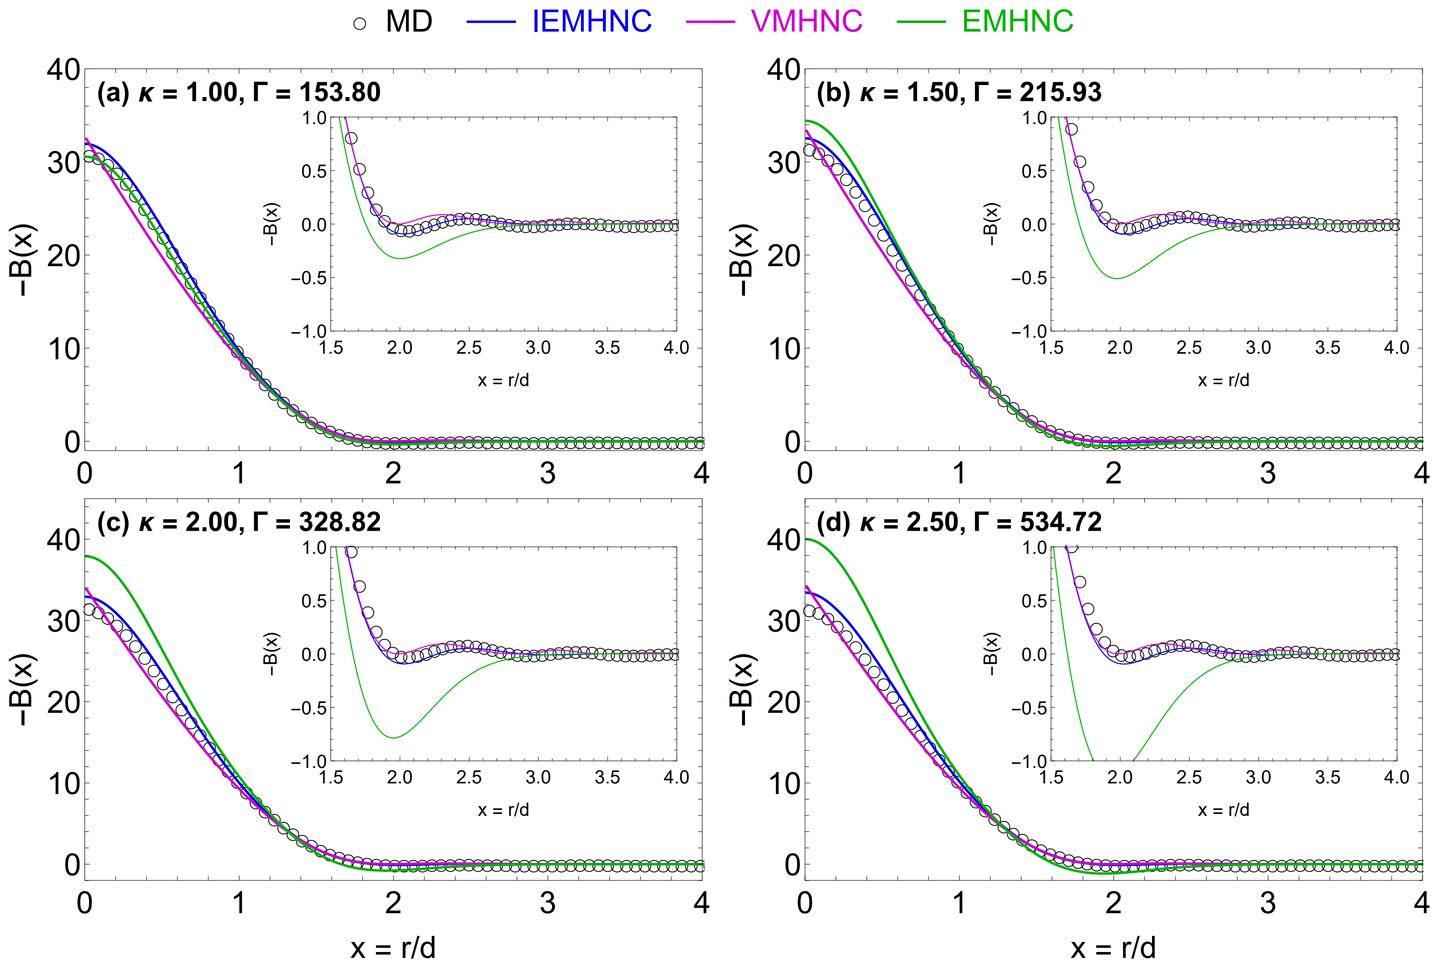


**Figure 2.** Bridge functions resulting from molecular dynamics (MD) simulations and from three integral equation theory approaches: the updated version of the isomorph-based empirically modified hypernetted chain approximation (IEMHNC) introduced in the present letter, the variational modified hypernetted-chain approximation (VMHNC) discussed in *G. Faussurier, Phys. Rev. E* **69***, 066402 (2004)* and the empirically modified hypernetted-chain approximation (EMHNC) presented in *W. Daughton, M. S. Murillo and L. Thode, Phys. Rev. E* **61***, 2129 (2000)*. The MD results are adopted from *F. Lucco Castello, P. Tolias and J. C. Dyre, J. Chem. Phys.* **154***, 034501 (2021)*. **Results for four YOCP state points that belong to the isomorphic line with reduced excess entropy $s_{\mathrm{ex}} = -3.380$.**

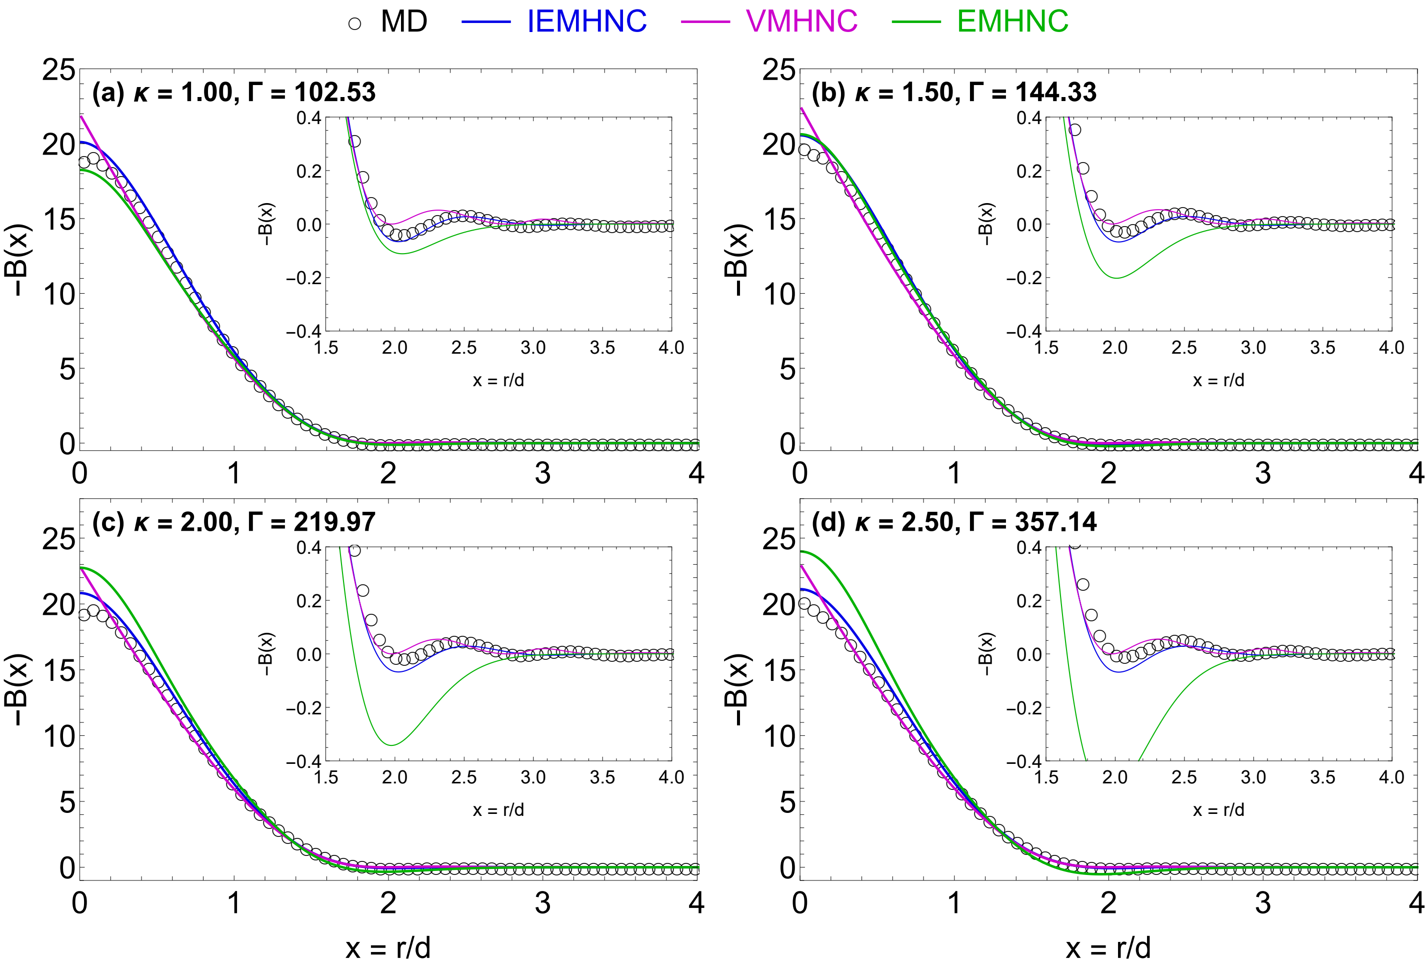


**Figure 3.** Bridge functions resulting from molecular dynamics (MD) simulations and from three integral equation theory approaches: the updated version of the isomorph-based empirically modified hypernetted chain approximation (IEMHNC) introduced in the present letter, the variational modified hypernetted-chain approximation (VMHNC) discussed in *G. Faussurier, Phys. Rev. E* **69**, *066402 (2004)* and the empirically modified hypernetted-chain approximation (EMHNC) presented in *W. Daughton, M. S. Murillo and L. Thode, Phys. Rev. E* **61**, *2129 (2000)*. The MD results are adopted from *F. Lucco Castello, P. Tolias and J. C. Dyre, J. Chem. Phys.* **154**, *034501 (2021)*. **Results for four YOCP state points that belong to the isomorphic line with reduced excess entropy $s_{\rm ex} = -2.764$.**

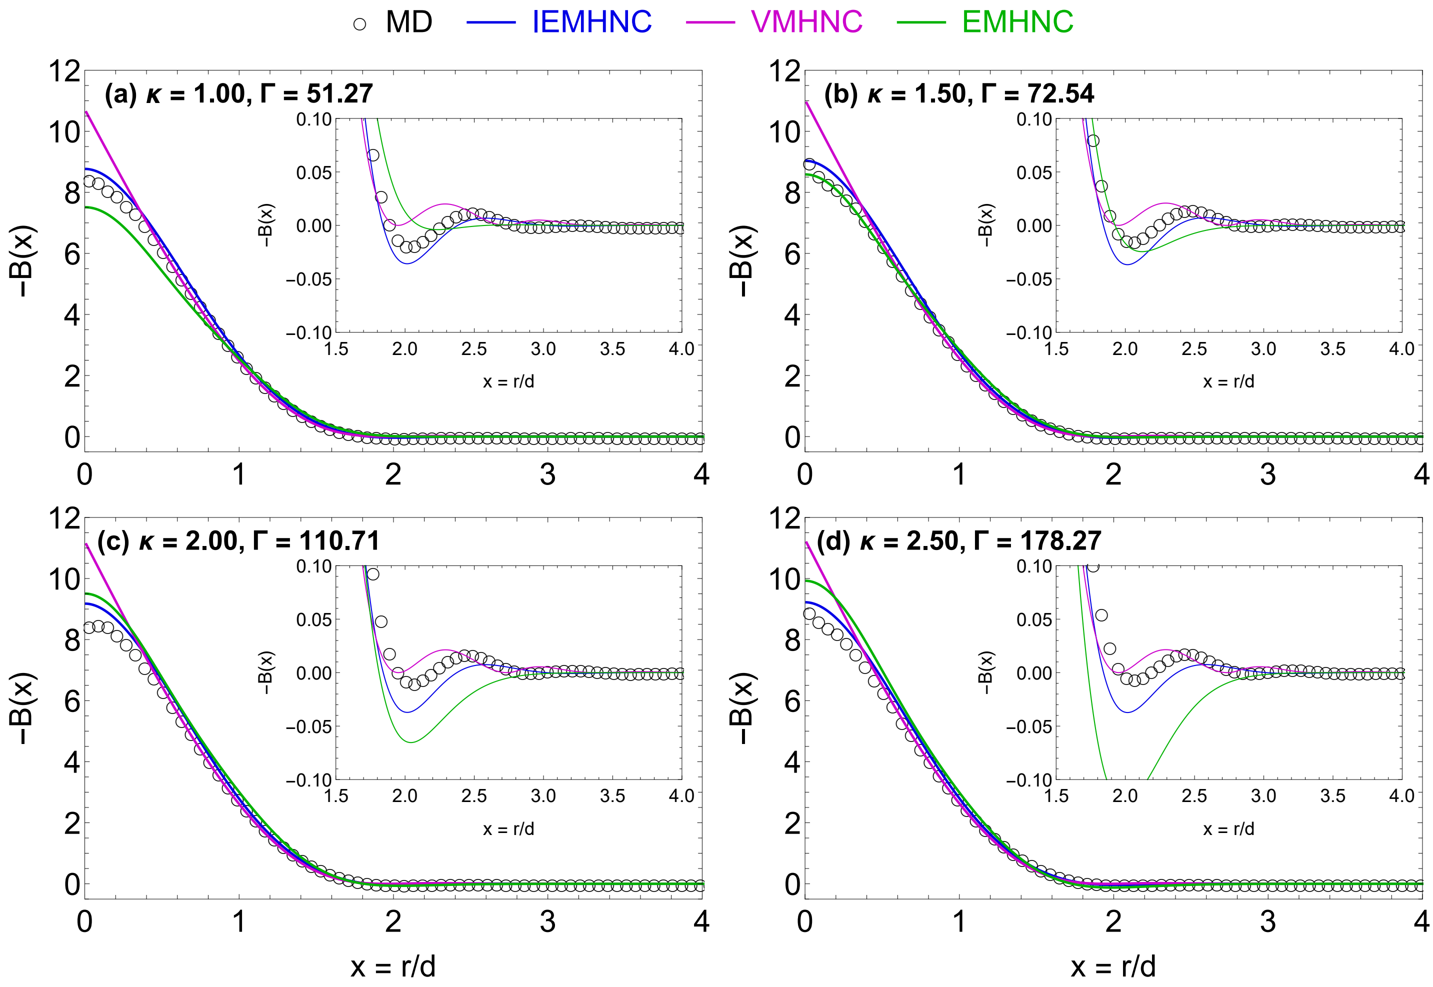


**Figure 4.** Bridge functions resulting from molecular dynamics (MD) simulations and from three integral equation theory approaches: the updated version of the isomorph-based empirically modified hypernetted chain approximation (IEMHNC) introduced in the present letter, the variational modified hypernetted-chain approximation (VMHNC) discussed in *G. Faussurier, Phys. Rev. E* **69**, *066402 (2004)* and the empirically modified hypernetted-chain approximation (EMHNC) presented in *W. Daughton, M. S. Murillo and L. Thode, Phys. Rev. E* **61**, *2129 (2000)*. The MD results are adopted from *F. Lucco Castello, P. Tolias and J. C. Dyre, J. Chem. Phys.* **154**, *034501 (2021)*. **Results for four YOCP state points that belong to the isomorphic line with reduced excess entropy $s_{\mathrm{ex}} = -1.918$.**

**Table 8.** Interaction energy $\widetilde{u} = (\pi\lambda r_s)^{-1} \int_0^\infty [S(x) - 1]\, dx$ (in Hartree units) of the unpolarized electron liquid as resulting from path integral Monte Carlo simulations (PIMC) after finite-size correction and from three theoretical approaches: the classical mapping method (CHNC) introduced in *M. W. C. Dharma-wardana and F. Perrot, Phys. Rev. Lett.* **84**, *959 (2000)*, the hypernetted-chain approach based dielectric scheme (HNC-STLS) introduced in *S. Tanaka, J. Chem. Phys.* **145**, *214104 (2016)* and the integral equation theory based dielectric scheme (IET-STLS) introduced in the present letter. The absolute relative deviations $\epsilon_r$ between the theoretical and the simulation results are also reported. The PIMC data for the first six states are adopted from *T. Dornheim, T. Sjostrom, S. Tanaka and J. Vorberger, Phys. Rev. B* **101**, *045129 (2020)*, whereas the PIMC data for the remaining 14 states are new.

| $r_s$ | $\theta$ | $\widetilde{u}$ PIMC | $\widetilde{u}$ CHNC | $e_{\mathrm{CHNC}}$ (%) | $\widetilde{u}$ HNC-STLS | $e_{\mathrm{HNC}}$ (%) | $\widetilde{u}$ IET-STLS | $e_{\mathrm{IET}}$ (%) |
|---|---|---|---|---|---|---|---|---|
| 100 | 0.50 | -0.00825500 | -0.00851455 | 3.144 | -0.00815866 | 1.167 | -0.00822181 | 0.402 |
| 100 | 0.75 | -0.00824570 | -0.00849036 | 2.967 | -0.00816490 | 0.980 | -0.00822544 | 0.246 |
| 100 | 1.00 | -0.00823490 | -0.00846118 | 2.748 | -0.00816618 | 0.834 | -0.00822559 | 0.113 |
| 100 | 2.00 | -0.00817650 | -0.00832747 | 1.846 | -0.00812905 | 0.580 | -0.00819066 | 0.173 |
| 100 | 4.00 | -0.00800623 | -0.00807606 | 0.872 | -0.00796833 | 0.473 | -0.00803143 | 0.315 |
| 50 | 0.50 | -0.01600700 | -0.01628910 | 1.762 | -0.01589841 | 0.678 | -0.01603510 | 0.176 |
| 60 | 0.50 | -0.01345310 | -0.01373697 | 2.110 | -0.01334804 | 0.781 | -0.01346014 | 0.052 |
| 70 | 0.50 | -0.01161175 | -0.01189556 | 2.444 | -0.01150938 | 0.882 | -0.01160390 | 0.068 |
| 80 | 0.50 | -0.01021937 | -0.01049969 | 2.743 | -0.01012012 | 0.971 | -0.01020149 | 0.175 |
| 90 | 0.50 | -0.00912862 | -0.00940208 | 2.996 | -0.00903293 | 1.048 | -0.00910415 | 0.268 |
| 110 | 0.50 | -0.00752642 | -0.00778104 | 3.383 | -0.00744012 | 1.147 | -0.00749675 | 0.394 |
| 125 | 0.50 | -0.00665421 | -0.00689090 | 3.557 | -0.00657377 | 1.209 | -0.00662268 | 0.474 |
| 125 | 0.75 | -0.00665053 | -0.00686927 | 3.289 | -0.00657838 | 1.085 | -0.00662556 | 0.442 |
| 125 | 1.00 | -0.00664336 | -0.00684417 | 3.023 | -0.00657999 | 0.954 | -0.00662647 | 0.254 |
| 125 | 1.50 | -0.00662535 | -0.00679058 | 2.494 | -0.00657432 | 0.770 | -0.00662112 | 0.064 |
| 125 | 2.00 | -0.00660298 | -0.00673751 | 2.037 | -0.00655900 | 0.666 | -0.00660712 | 0.063 |
| 150 | 0.50 | -0.00558177 | -0.00578664 | 3.670 | -0.00550821 | 1.318 | -0.00554797 | 0.606 |
| 150 | 1.00 | -0.00557134 | -0.00574482 | 3.114 | -0.00551337 | 1.040 | -0.00555132 | 0.359 |
| 200 | 0.50 | -0.00422244 | -0.00437922 | 3.713 | -0.00416445 | 1.373 | -0.00419373 | 0.680 |
| 200 | 1.00 | -0.00421710 | -0.00434573 | 3.050 | -0.00416813 | 1.161 | -0.00419559 | 0.510 |
